# Supplementary material for: Training Dataset Matters for Machine Learning Interatomic Potentials: Water Simulation as an Example
Source: arXiv:2512.23939 source file (2026-10-12)
Supplement: Supplementary file 1 [file sm.tex]

\documentclass[%
 % reprint,
superscriptaddress,
%groupedaddress,
%unsortedaddress,
%runinaddress,
%frontmatterverbose, 
% preprint,
%preprintnumbers,
%nofootinbib,
%nobibnotes,
%bibnotes,
 amsmath,amssymb,
 aps,
 % prl,
%pra,
% prb,
%rmp,
%prstab,
%prstper,
%floatfix,
% twocolumn=false,
]{revtex4-2}
\usepackage{xr}
\externaldocument{main}

\usepackage[T1]{fontenc}
\usepackage{tgtermes}

\usepackage{array}
\usepackage{subcaption}
\usepackage{caption}
\usepackage{cleveref}

% Custom label format for Supplementary Information
\DeclareCaptionLabelFormat{supp}{#1 #2}
\captionsetup[table]{labelformat=supp, labelsep=period, name=TABLE}
\captionsetup[figure]{labelformat=supp, labelsep=period, name=FIG.}

% Redefine \thetable and \thefigure for referencing

\usepackage{graphicx}% Include figure files
\usepackage{dcolumn}% Align table columns on decimal point
\usepackage{bm}% bold math
\usepackage{braket}
\usepackage{xcolor}
%\usepackage{hyperref}% add hypertext capabilities
%\usepackage[mathlines]{lineno}% Enable numbering of text and display math
%\linenumbers\relax % Commence numbering lines

%\usepackage[showframe,%Uncomment any one of the following lines to test 
%%scale=0.7, marginratio={1:1, 2:3}, ignoreall,% default settings
%%text={7in,10in},centering,
%%margin=1.5in,
%%total={6.5in,8.75in}, top=1.2in, left=0.9in, includefoot,
%%height=10in,a5paper,hmargin={3cm,0.8in},
%]{geometry}

\begin{document}

% \preprint{APS/123-QED}
% \input{main.tex}
% \title{Supplemental Material for\\ \maintitle}
\title{Supplemental Material for\\Ab Initio Melting Properties of Water and Ice from Machine Learning Potentials Simulations}% Force line breaks with \\
% \thanks{A footnote to the article title}%
\author{Yifan Li}
\affiliation{ 
Department of Chemistry, Princeton University, Princeton, NJ 08544, USA%\\This line break forced with \textbackslash\textbackslash
}%
 % \altaffiliation[Also at ]{Physics Department, XYZ University.}%Lines break automatically or can be forced with \\
\author{Bingjia Yang}%
\affiliation{ 
Department of Chemistry, Princeton University, Princeton, NJ 08544, USA%\\This line break forced with \textbackslash\textbackslash
}%
\author{Chunyi Zhang}
\affiliation{ 
Eastern Institute of Technology, Ningbo, Zhejiang 315200, China
% Department of Chemistry, Princeton University, Princeton, NJ 08544, USA%\\This line break forced with \textbackslash\textbackslash
}%
\author{Axel Gomez}
\affiliation{ 
Department of Chemistry, Princeton University, Princeton, NJ 08544, USA%\\This line break forced with \textbackslash\textbackslash
}%
\author{Pinchen Xie}
\affiliation{ 
Program in Applied and Computational Mathematics, Princeton University, Princeton, NJ 08544, USA%\\This line break forced with \textbackslash\textbackslash
}
\author{Yixiao Chen}
\affiliation{ 
Program in Applied and Computational Mathematics, Princeton University, Princeton, NJ 08544, USA%\\This line break forced with \textbackslash\textbackslash
}
\author{Pablo M. Piaggi}
\affiliation{CIC nanoGUNE BRTA, Tolosa Hiribidea 76, 20018 Donostia-San Sebastián, Spain}
\affiliation{Ikerbasque, Basque Foundation for Science, 48013 Bilbao, Spain}

\author{Roberto Car}
 % \email{Second.Author@institution.edu.}
\affiliation{ 
Department of Chemistry, Princeton University, Princeton, NJ 08544, USA%\\This line break forced with \textbackslash\textbackslash
}%
\affiliation{ 
Program in Applied and Computational Mathematics, Princeton University, Princeton, NJ 08544, USA%\\This line break forced with \textbackslash\textbackslash
}
\affiliation{ 
Department of Physics, Princeton University, Princeton, NJ 08544, USA%\\This line break forced with \textbackslash\textbackslash
}%
\affiliation{ 
Princeton Institute for the Science and Technology of Materials, Princeton University, Princeton, NJ 08544, USA%\\This line break forced with \textbackslash\textbackslash
}%
\maketitle
\section{Deep Potential models}\label{sm_model}
% Here we describe how we trained our Deep Potential (DP) models. We first describe the settings of the DFT calculations, and then introduce the training dataset generated by the active learning approach. To conclude this section, we demonstrate the accuracy of the DP models for the four DFT functionals considered in the main text by reporting the corresponding training and test errors.

\subsection{Training Dataset}\label{sm_modeldataset}
% We use DeePMD-kit\cite{wang_deepmd-kit_2018, zeng_deepmd-kit_2023} to train four DP models for these DFT functionals. We use the se\_e2\_a descriptor\cite{han_deep_2018, zhang_deep_2018, zhang_end--end_2018} and choose a 6 \AA cutoff radius for the model.
The overall number of training data of each DP model is summarized in Table \ref{dataset}.

\begin{table}[h!]
\caption{The Composition of Dataset of Each Model}
% \begin{tabular}{m{3cm}p{3cm}p{3cm}p{3cm}}
\begin{tabular}{cccccc}
\hline
Functional & Classical Water & Quantum Water & Classical Ice & Quantum Ice & Total \\ \hline
revPBE-D3 &  4142  &     720  &   385 & 686  &  5933  \\
revPBE0-D3  & 179 & 749 & 3 & 847 & 1778 \\
SCAN   & 1 & 3553 & 0 &   1153   &  4707 \\
SCAN0  & 0 &  7749 &  0 &  96 & 7845 \\ \hline
\end{tabular}%
\label{dataset}
\end{table}

% We want to point out that the number of training data differs very much because we add different numbers of data into the dataset after the exploration stage for different models. The configurations added in a single iteration can be similar and selecting too many configurations in each iteration will lead to redundancy in the dataset. In the four models above, the revPBE0-D3 model has the most reasonable number of training data, and the other three datasets have more data than a minimum complete dataset.

\subsection{Training Error}
% With the training dataset that we have built in the last section, we report the accuracy of the training. The DFT energies and forces used for training are compared to the values predicted by the DP models in FIG. \ref{parity}. It shows that for each functional, the DP model has been accurately trained on the complete datasets generated in the last section.
In FIG. \ref{parity} energies and forces predicted by the four DP models are compared with the corresponding DFT values for the configurations in the training dataset. The resulting mean absolute error (MAE) and root mean square error (RMSE) are reported in TABLE \ref{error}.

% We also report the training mean absolute error (MAE) and root mean square error (RMSE) of each model in Table \ref{error}.

\begin{table}[h!]
\caption{The Training MAE and RMSE of Each Model}
% \begin{tabular}{m{3cm}p{3cm}p{3cm}p{3cm}}
\begin{tabular}{ccccc}
\hline
Model for Functional & Energy MAE [meV / atom]& Energy RMSE [meV / atom]& Force MAE [meV / \AA] & Force RMSE [meV / \AA] \\ \hline
revPBE-D3 & 0.289 & 0.372  & 27.3 & 36.0 \\
revPBE0-D3  & 0.300 & 0.388 & 28.0 & 37.0  \\
SCAN &  0.475 & 0.599 & 67.5 & 97.5 \\
SCAN0 & 0.667 & 0.825 & 52.5 & 71.6 \\ \hline
\end{tabular}%
\label{error}
\end{table}

% The carefully selected dataset and the low training error guarantee that our models faithfully reproduce DFT energies and forces of the configurations encountered in the production MD and PIMD tasks, and thus the melting points we calculated can represent the properties predicted by the DFT functionals we test.

\begin{figure}
   \centering
\begin{subfigure}[b]{0.45\linewidth}
\includegraphics[height=6cm]{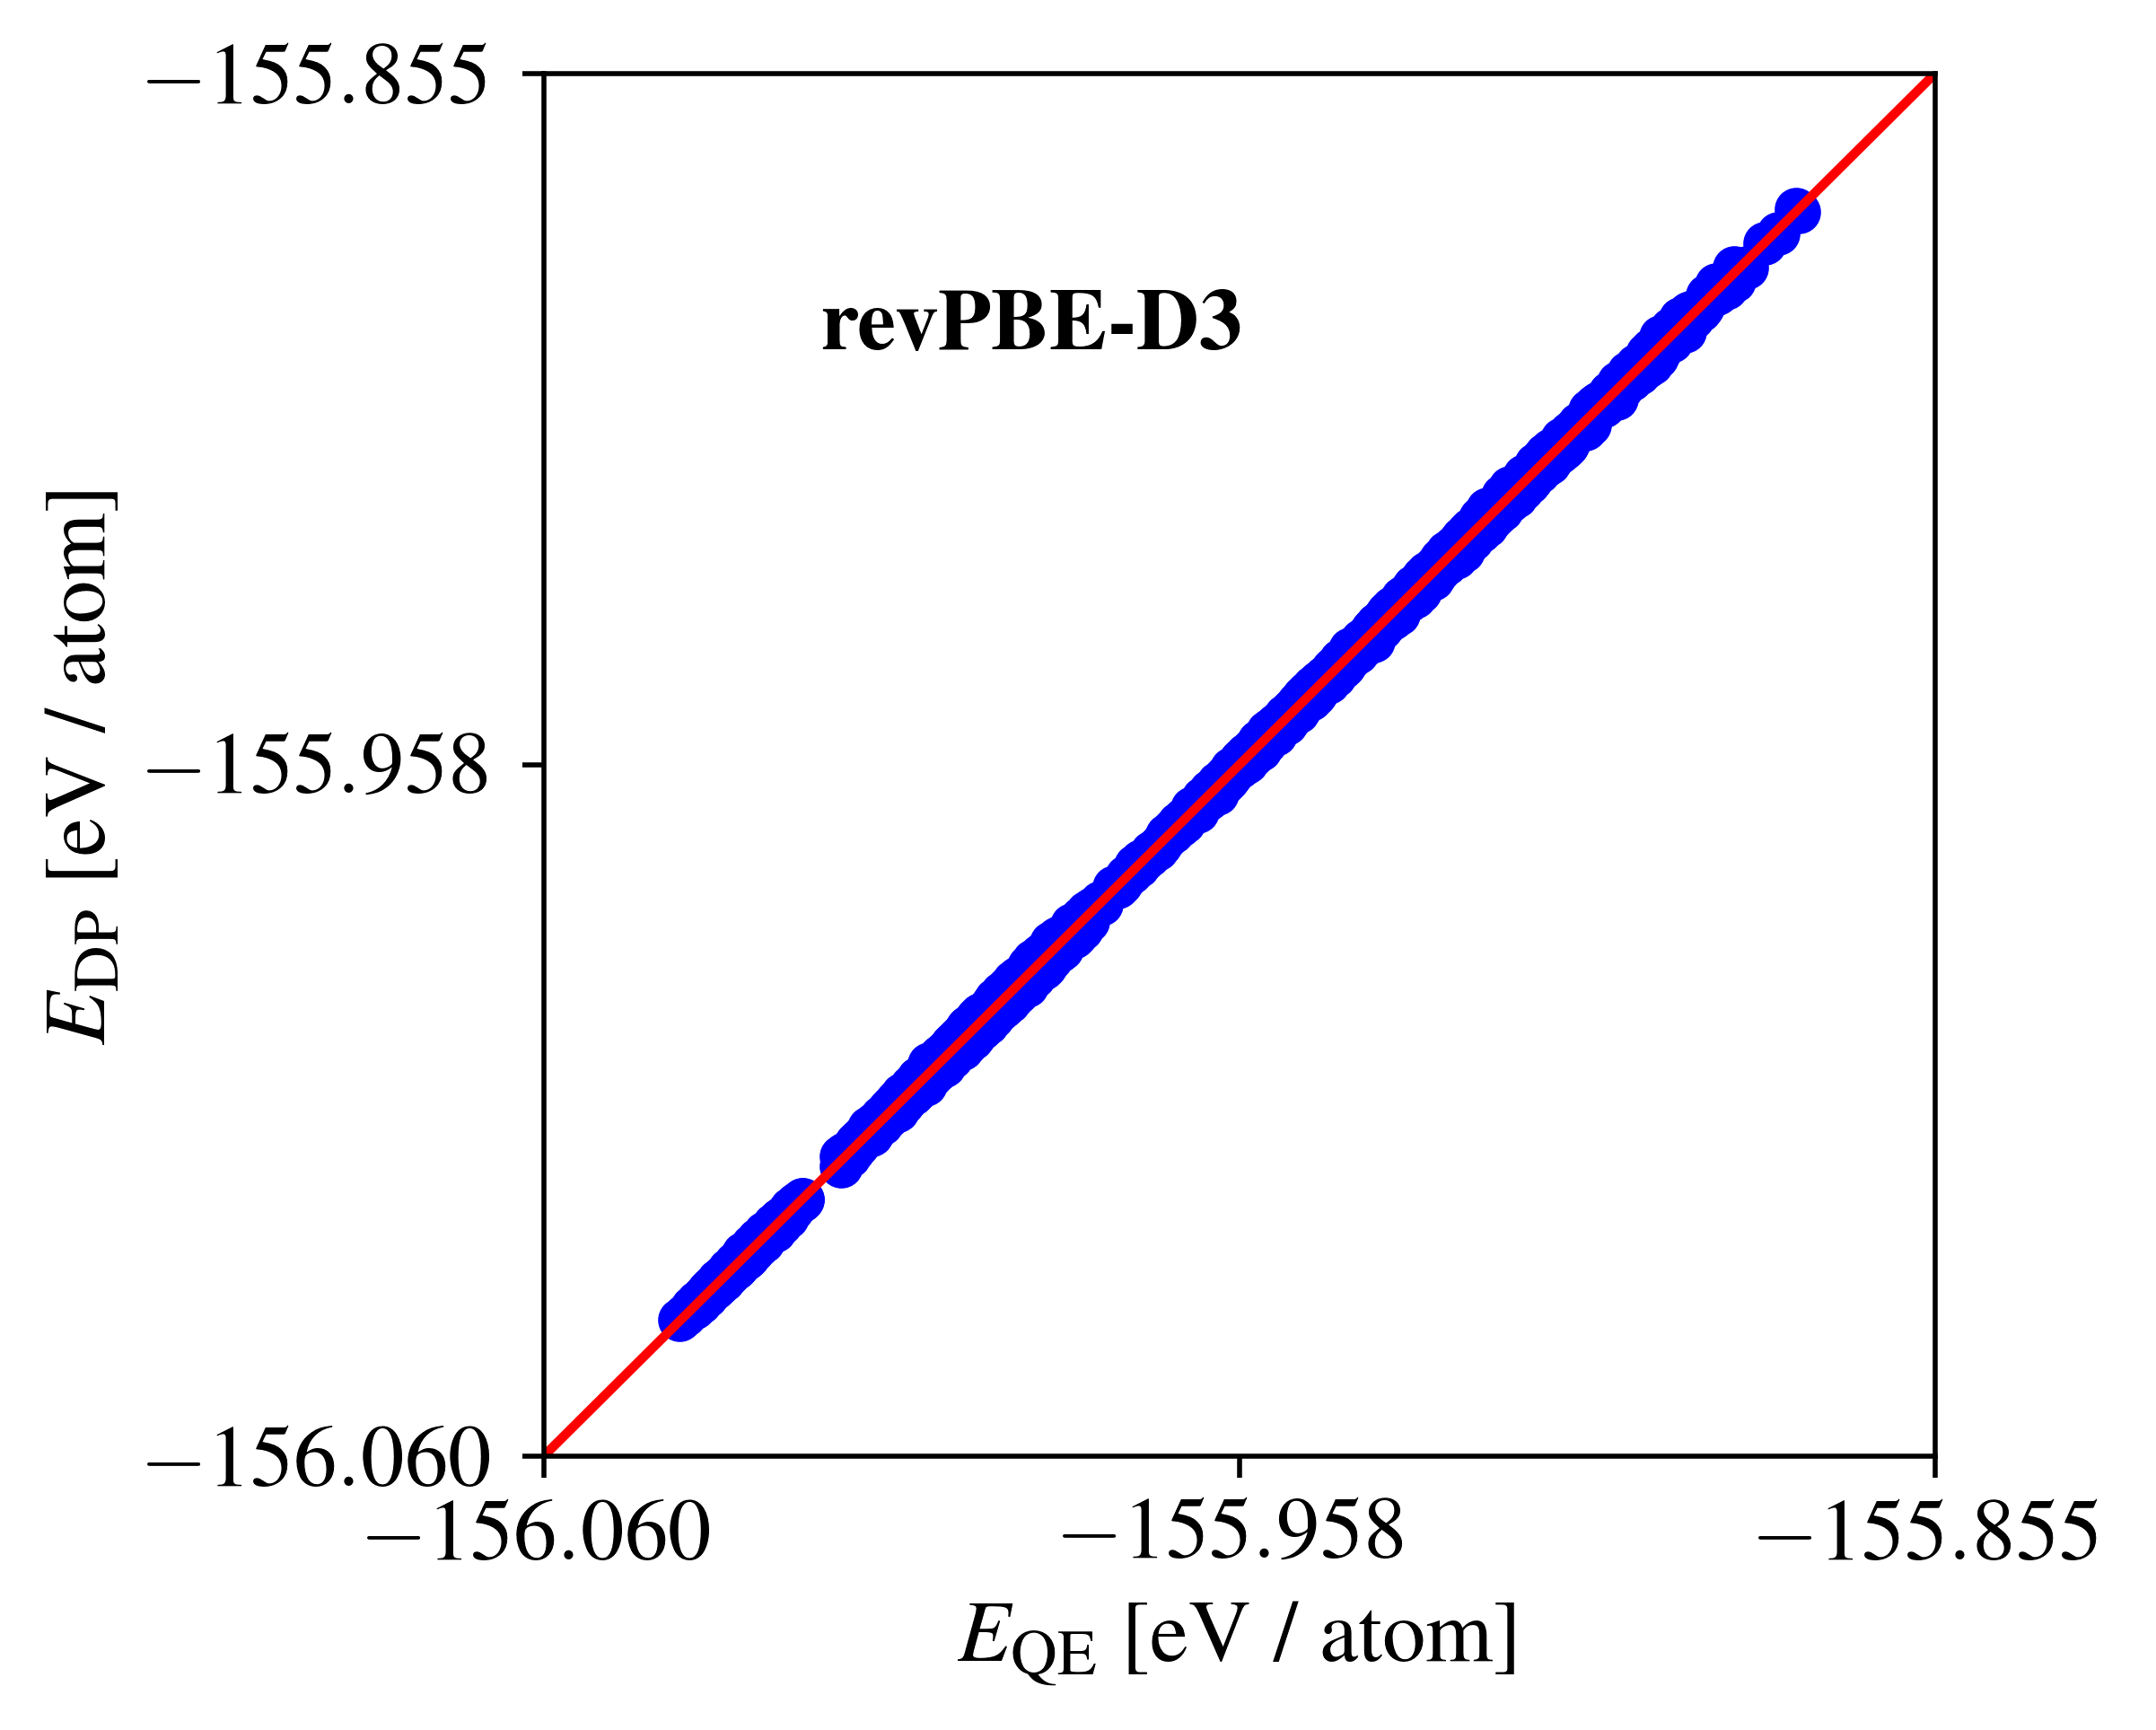}
\end{subfigure}
\hspace{0.1cm}
\begin{subfigure}[b]{0.45\linewidth}
\includegraphics[height=6cm]{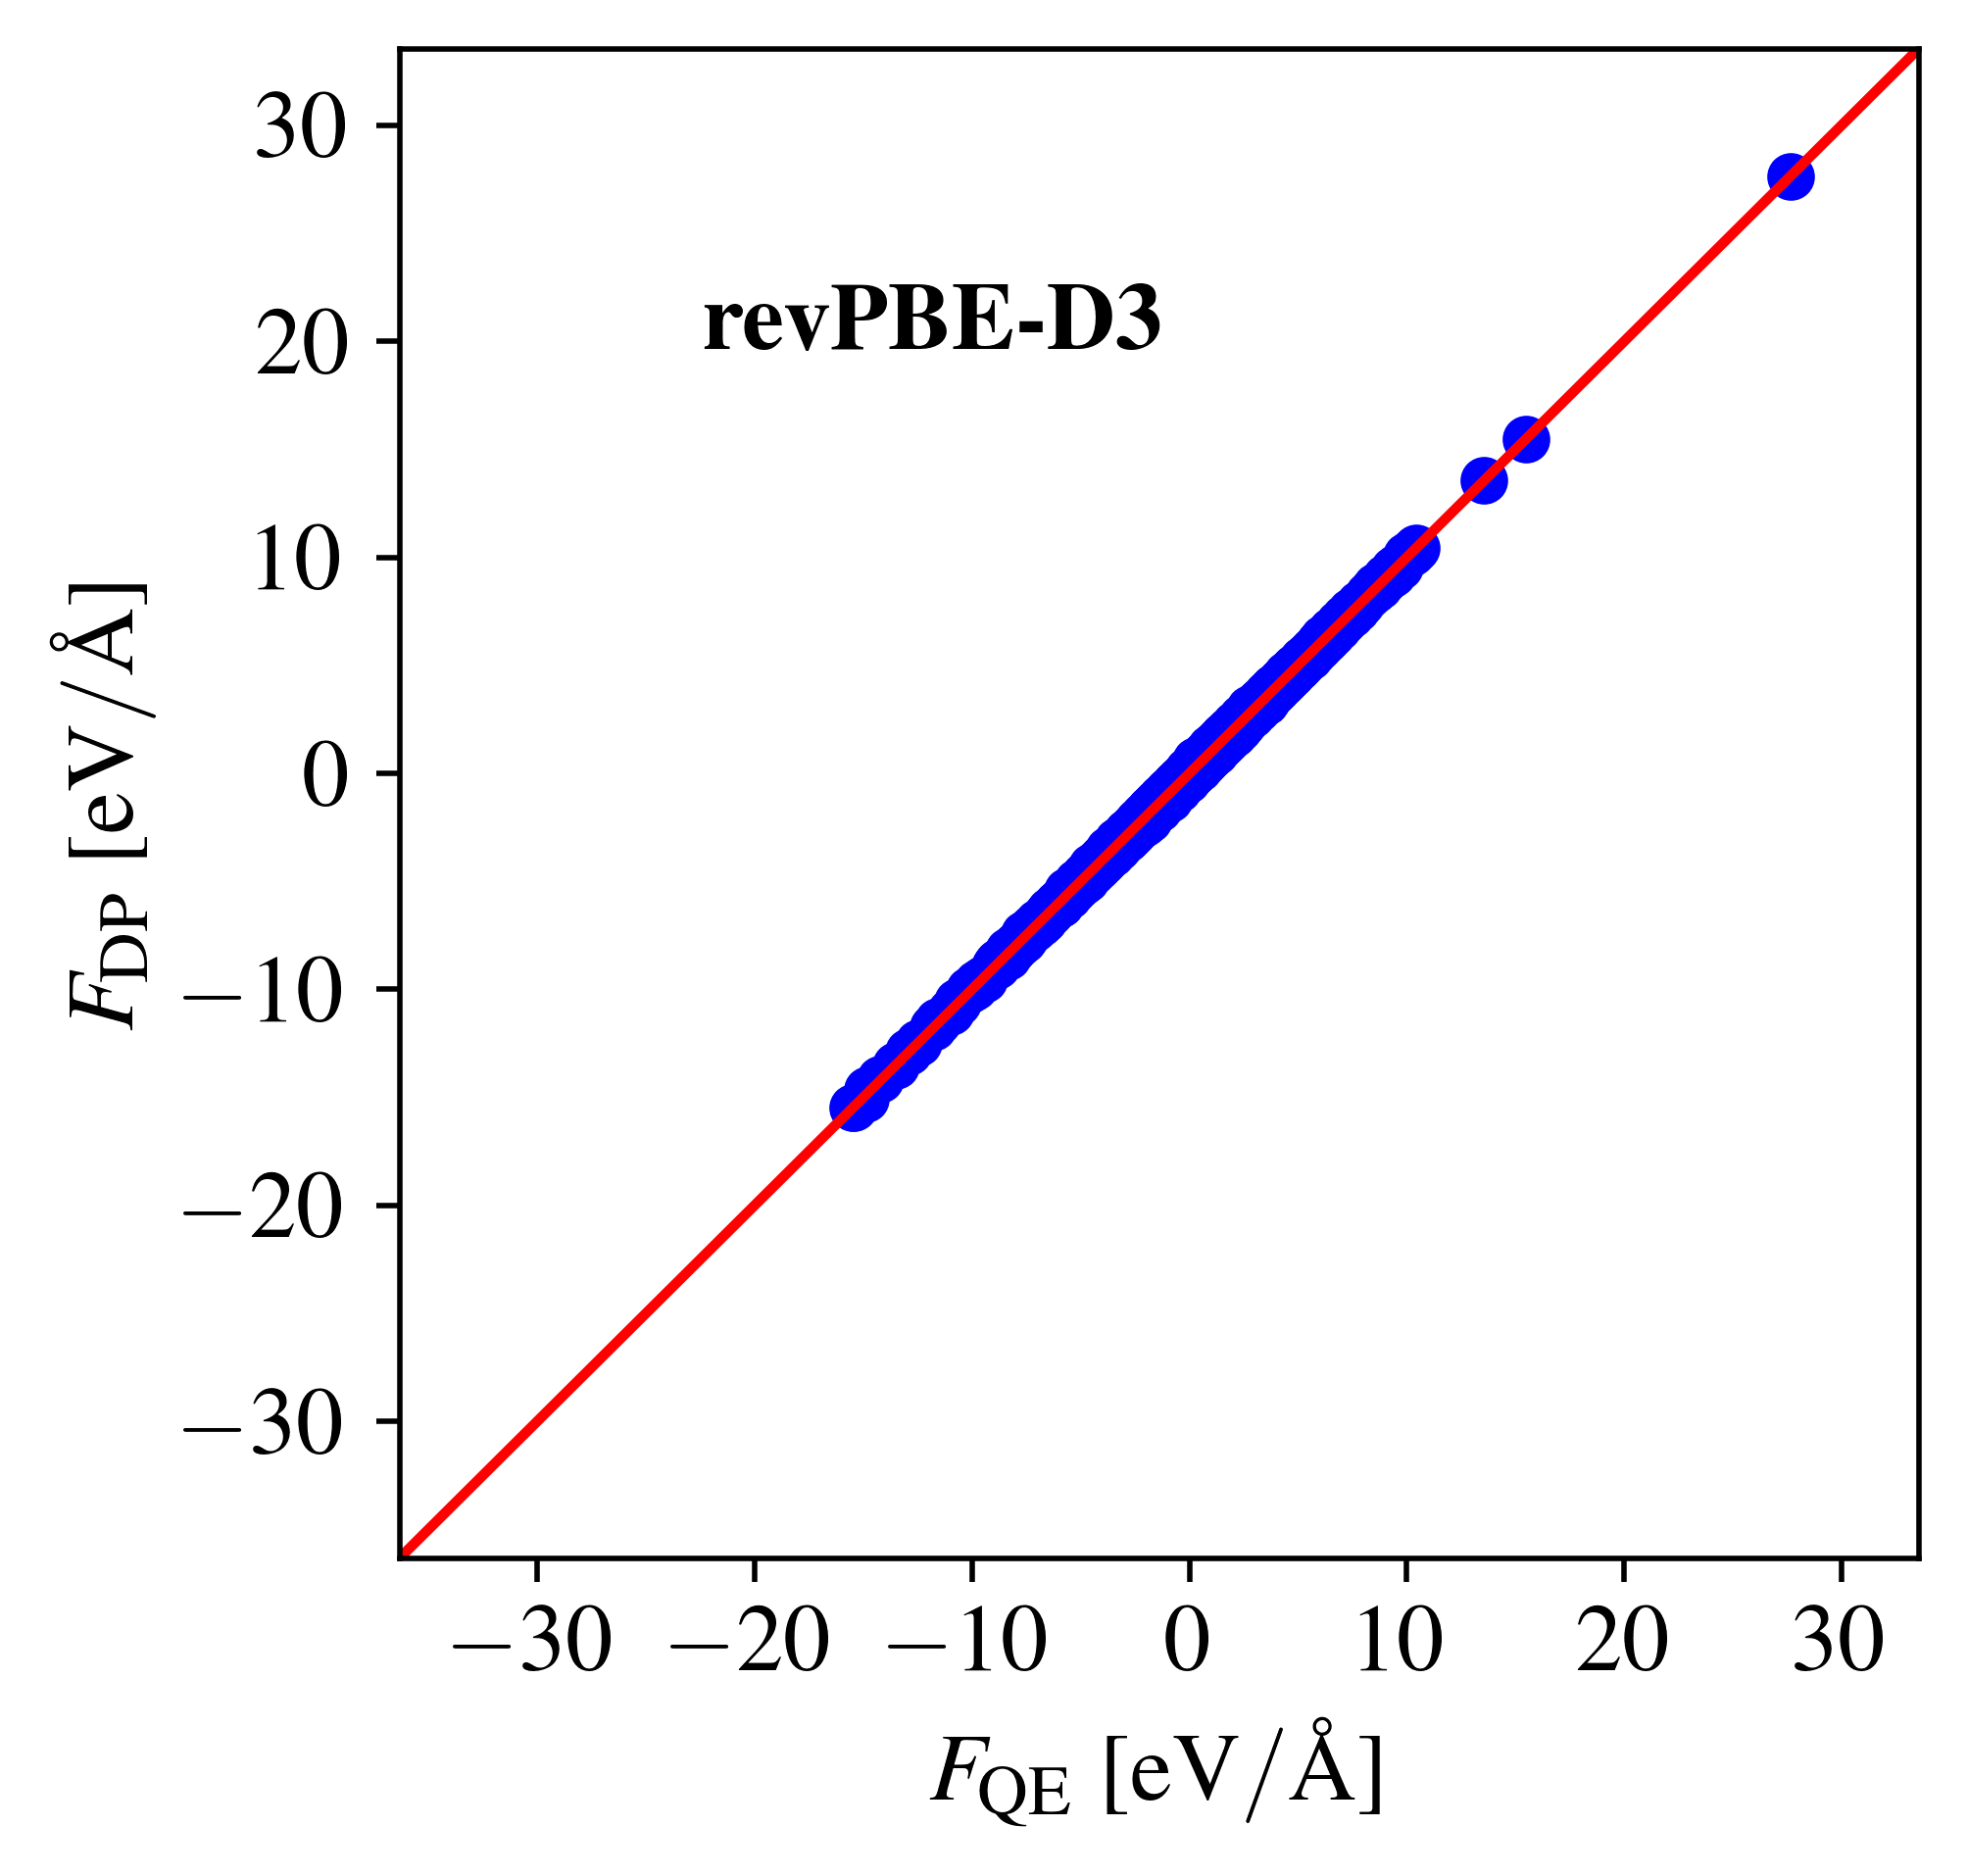}
\end{subfigure}

\vspace{0.1cm}

\begin{subfigure}[b]{0.45\linewidth}
\includegraphics[height=6cm]{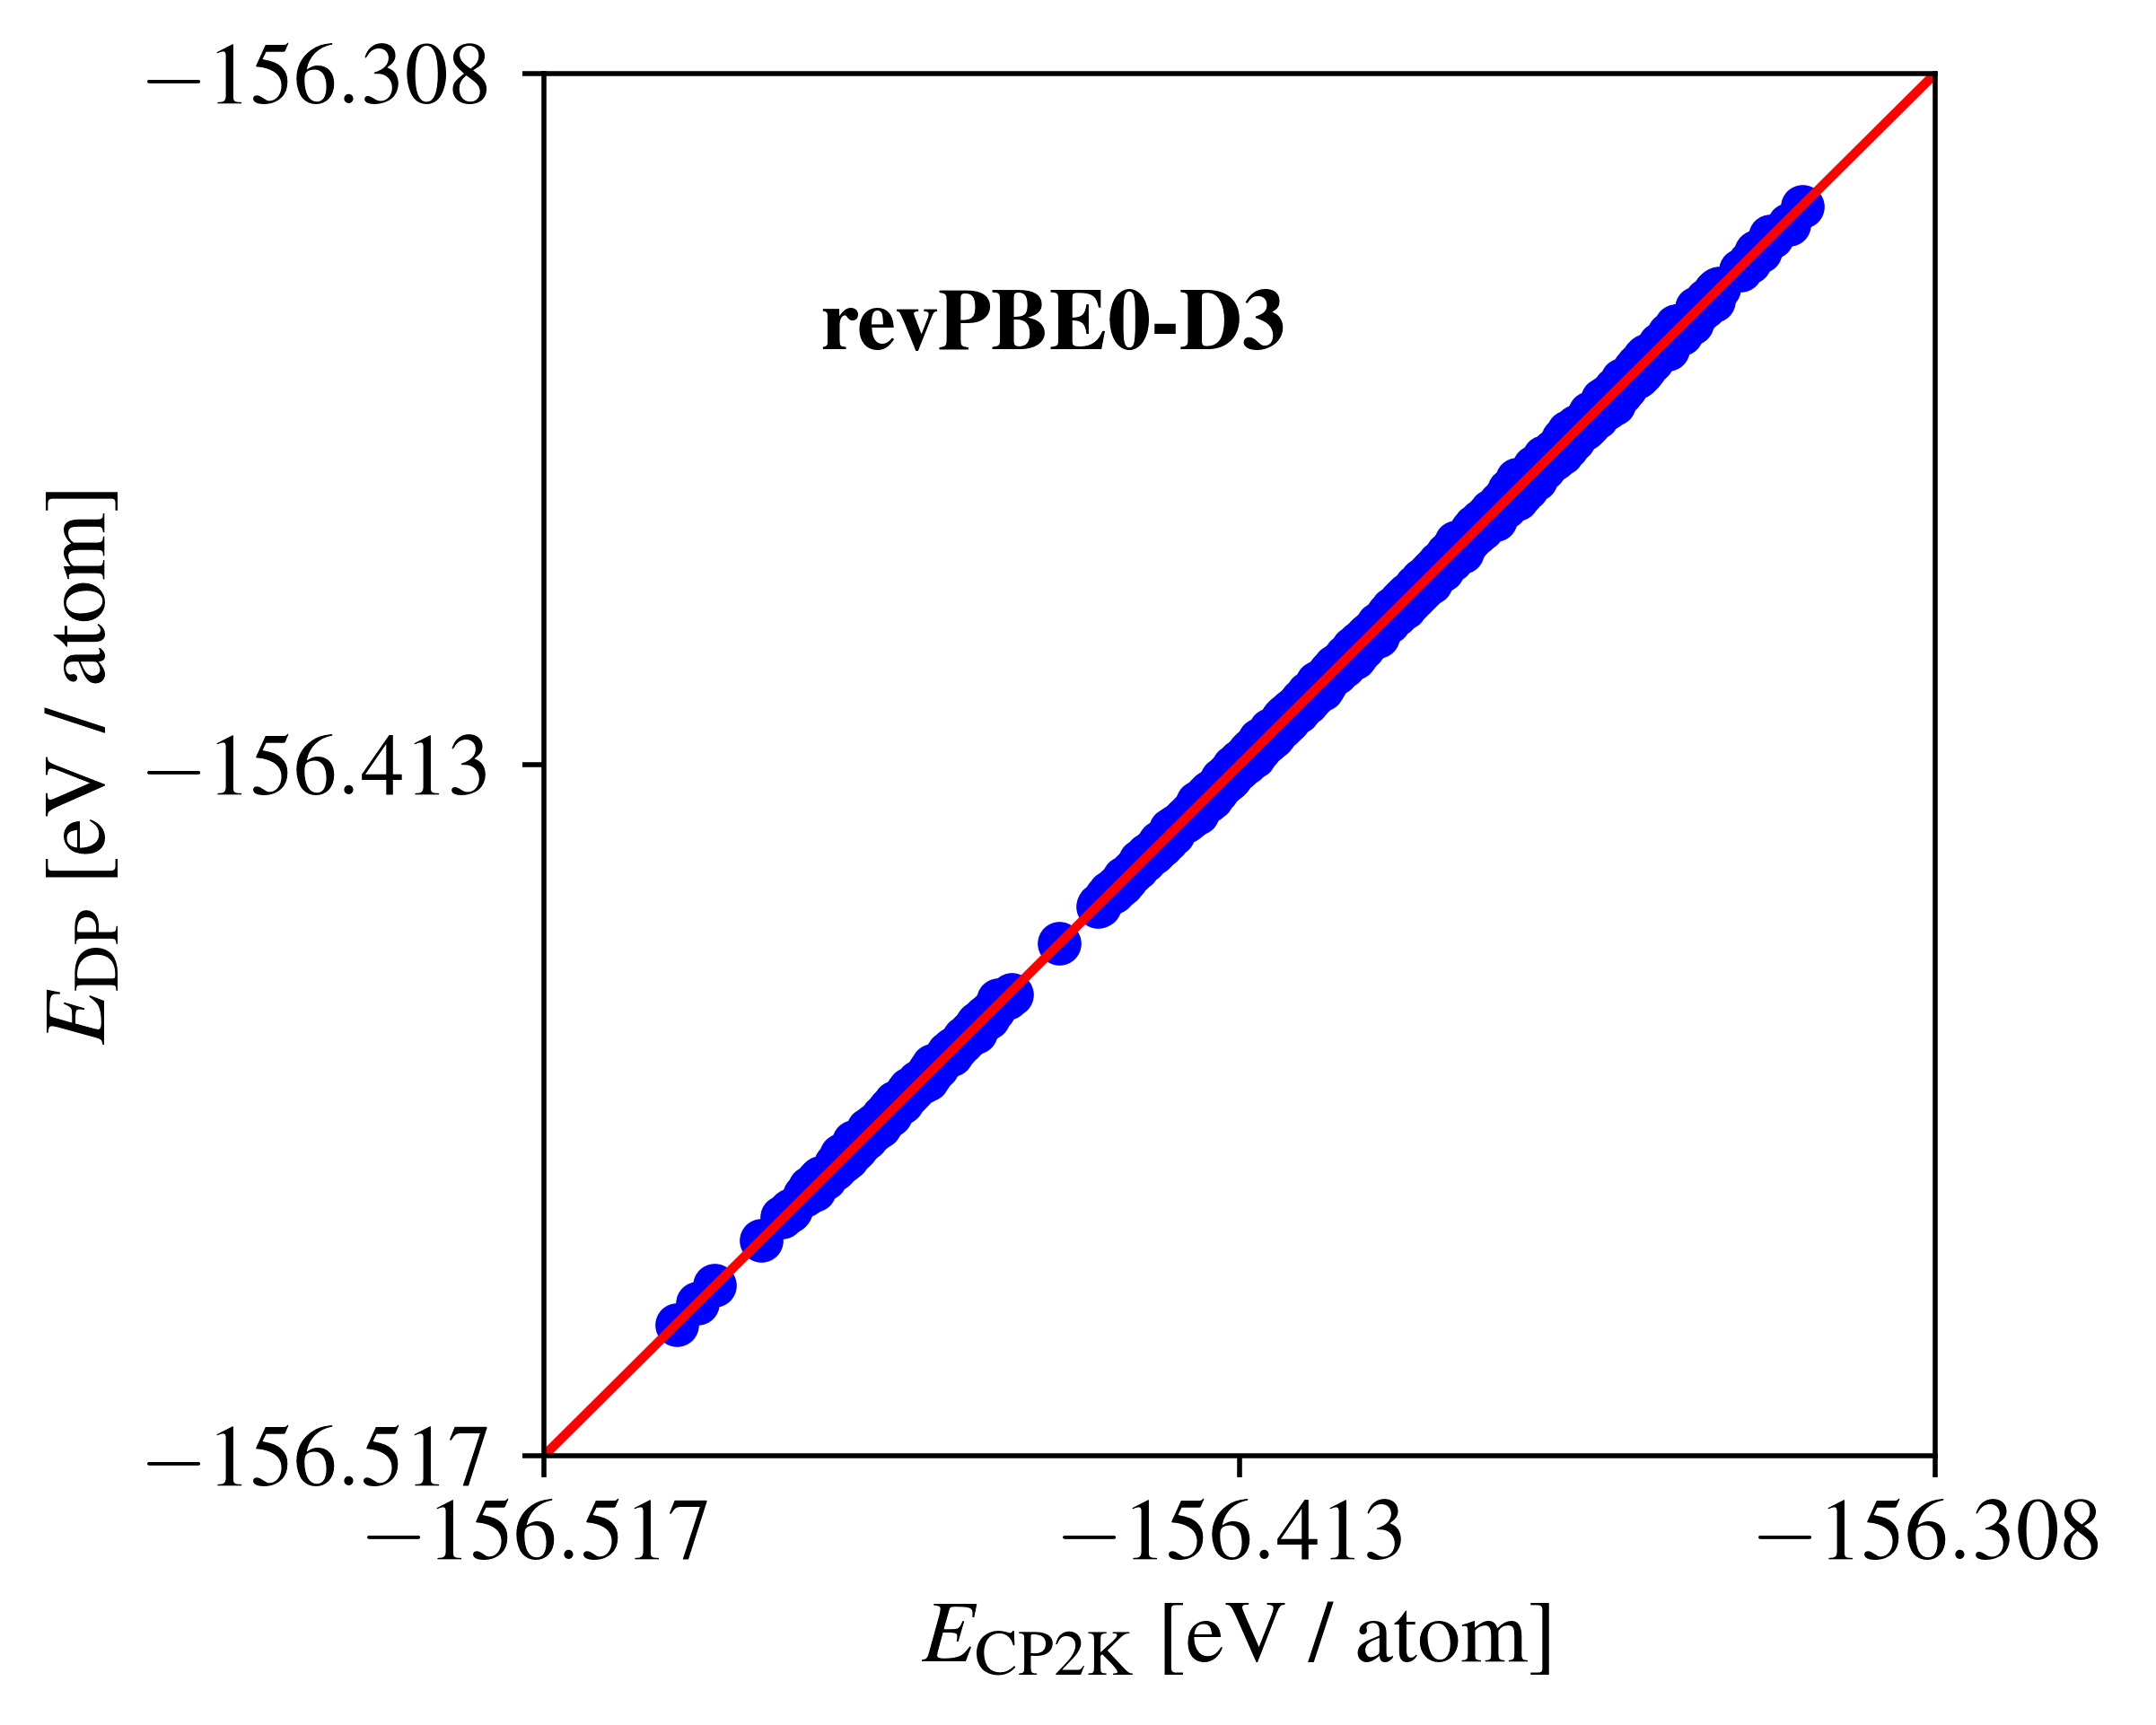}
\end{subfigure}
\hspace{0.1cm}
\begin{subfigure}[b]{0.45\linewidth}
\includegraphics[height=6cm]{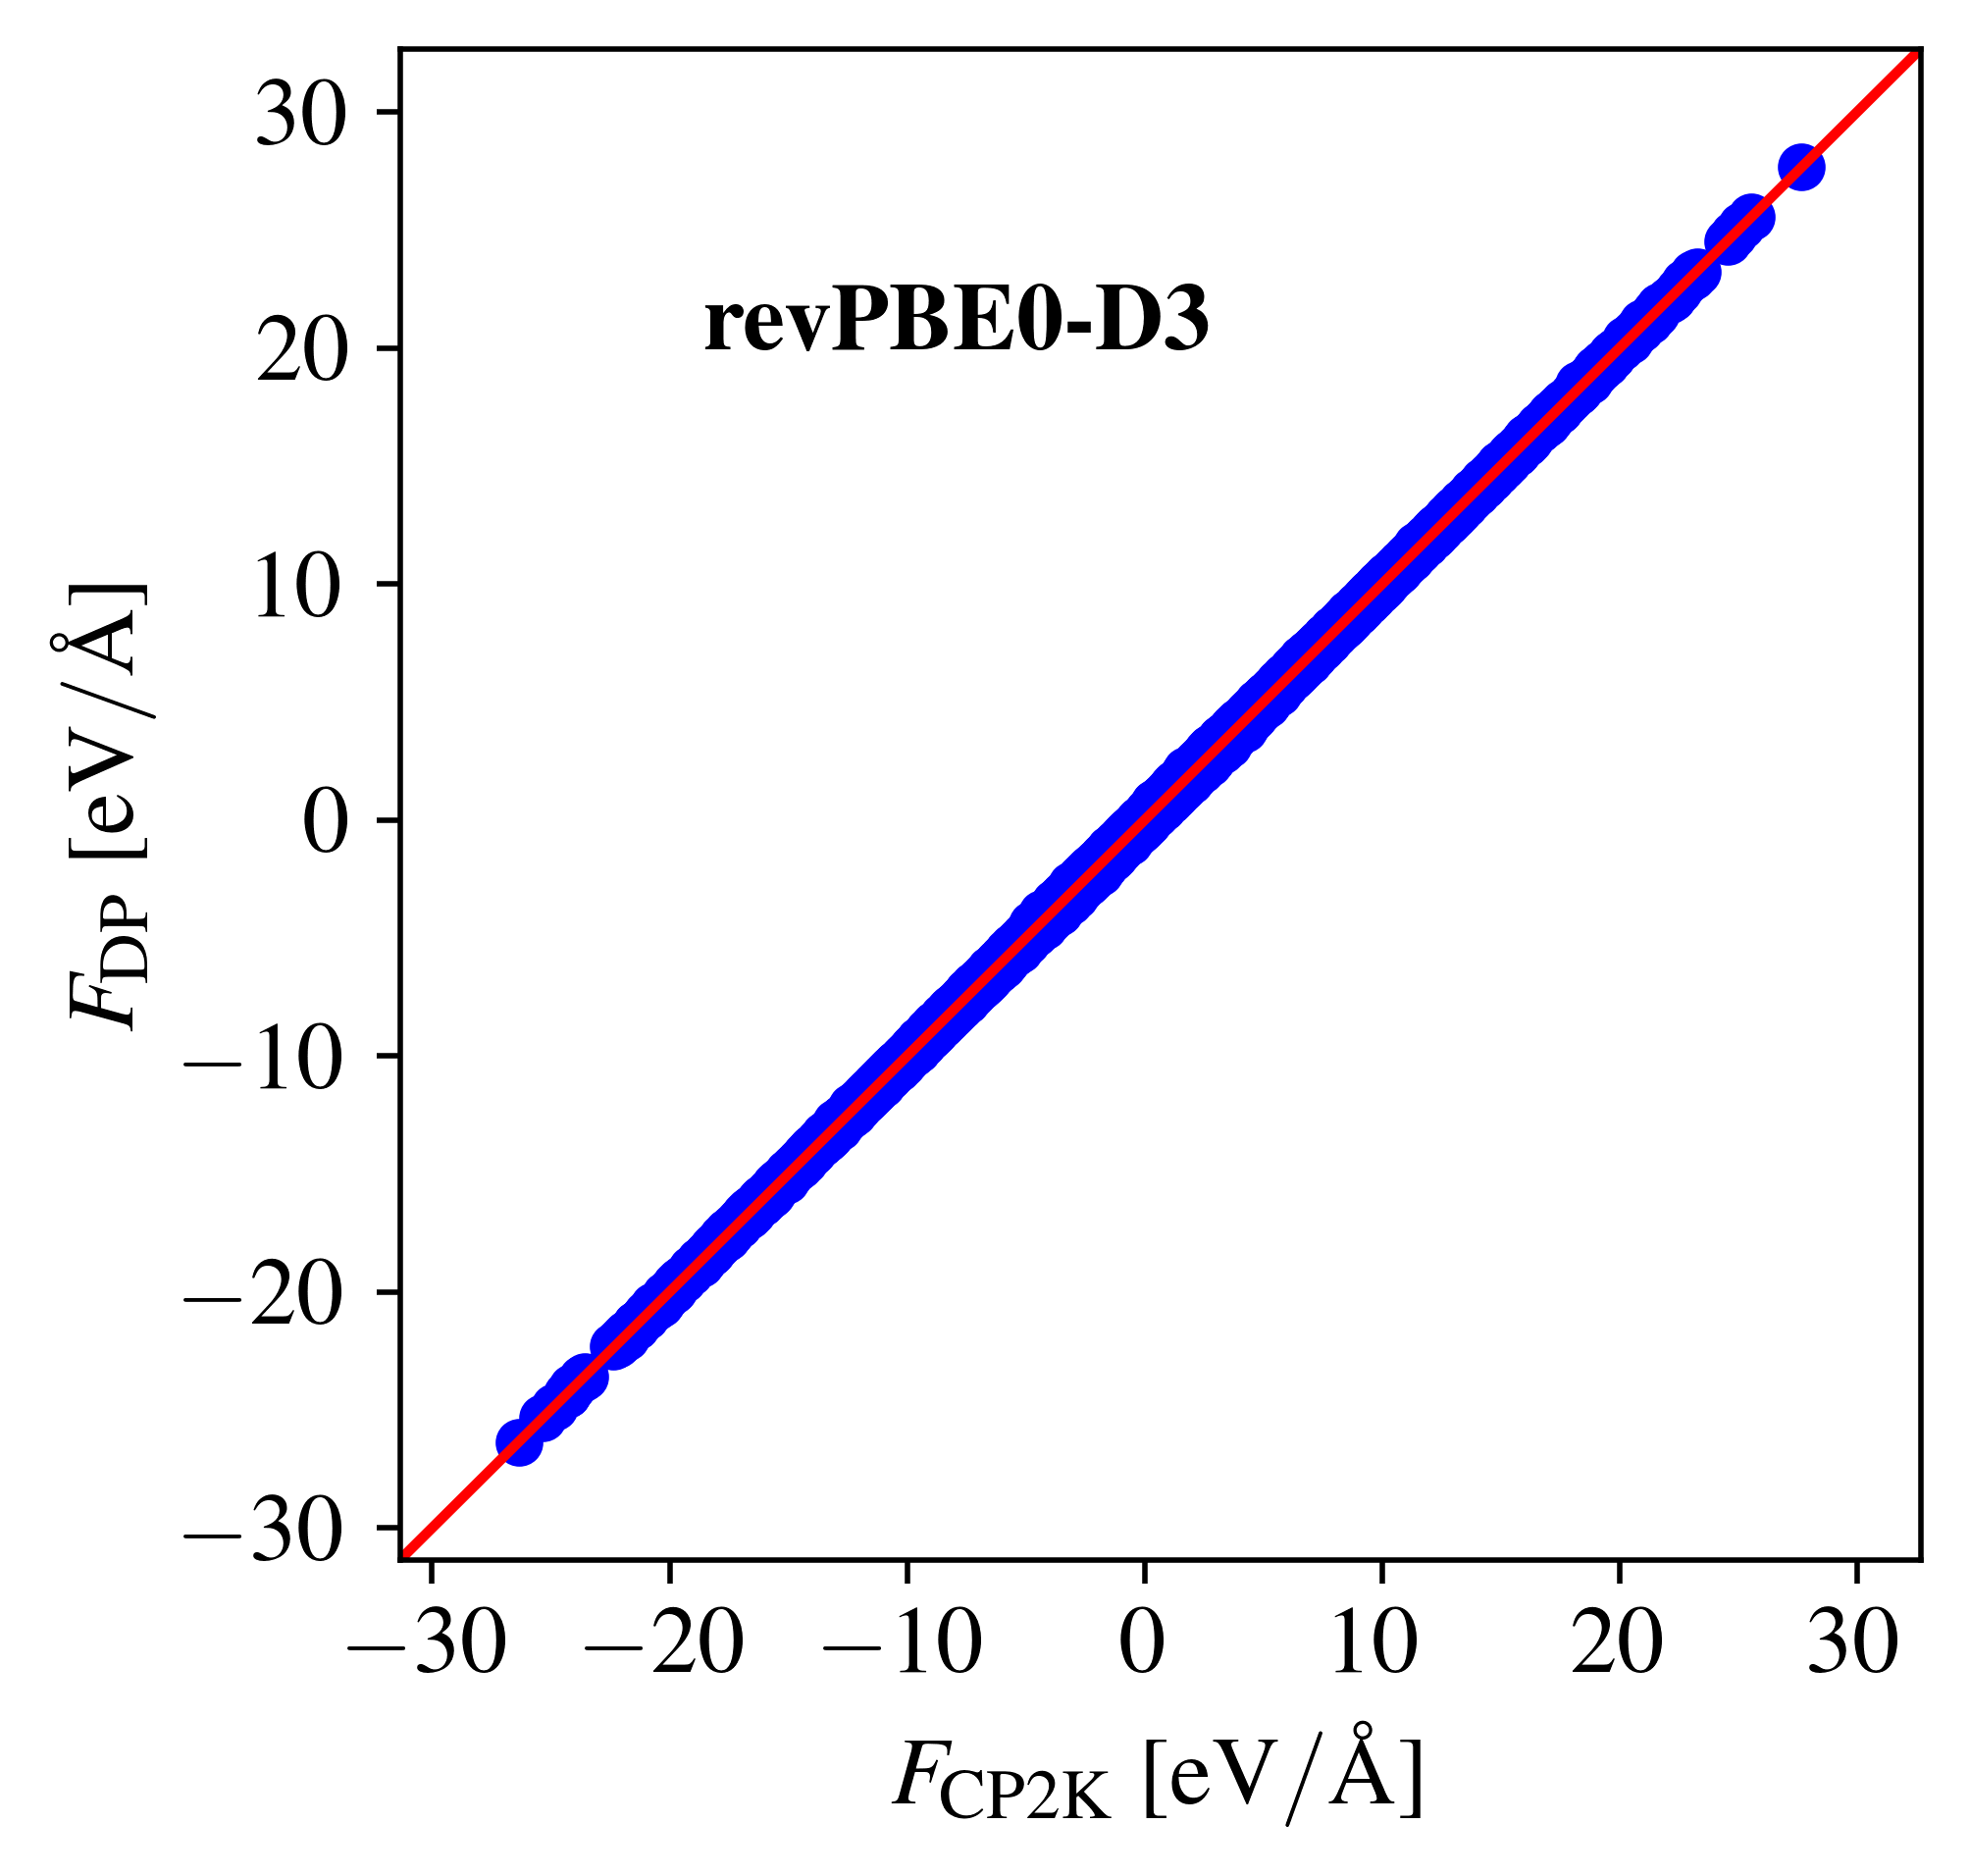}
\end{subfigure}

\vspace{0.1cm}

\begin{subfigure}[b]{0.45\linewidth}
\includegraphics[height=6cm]{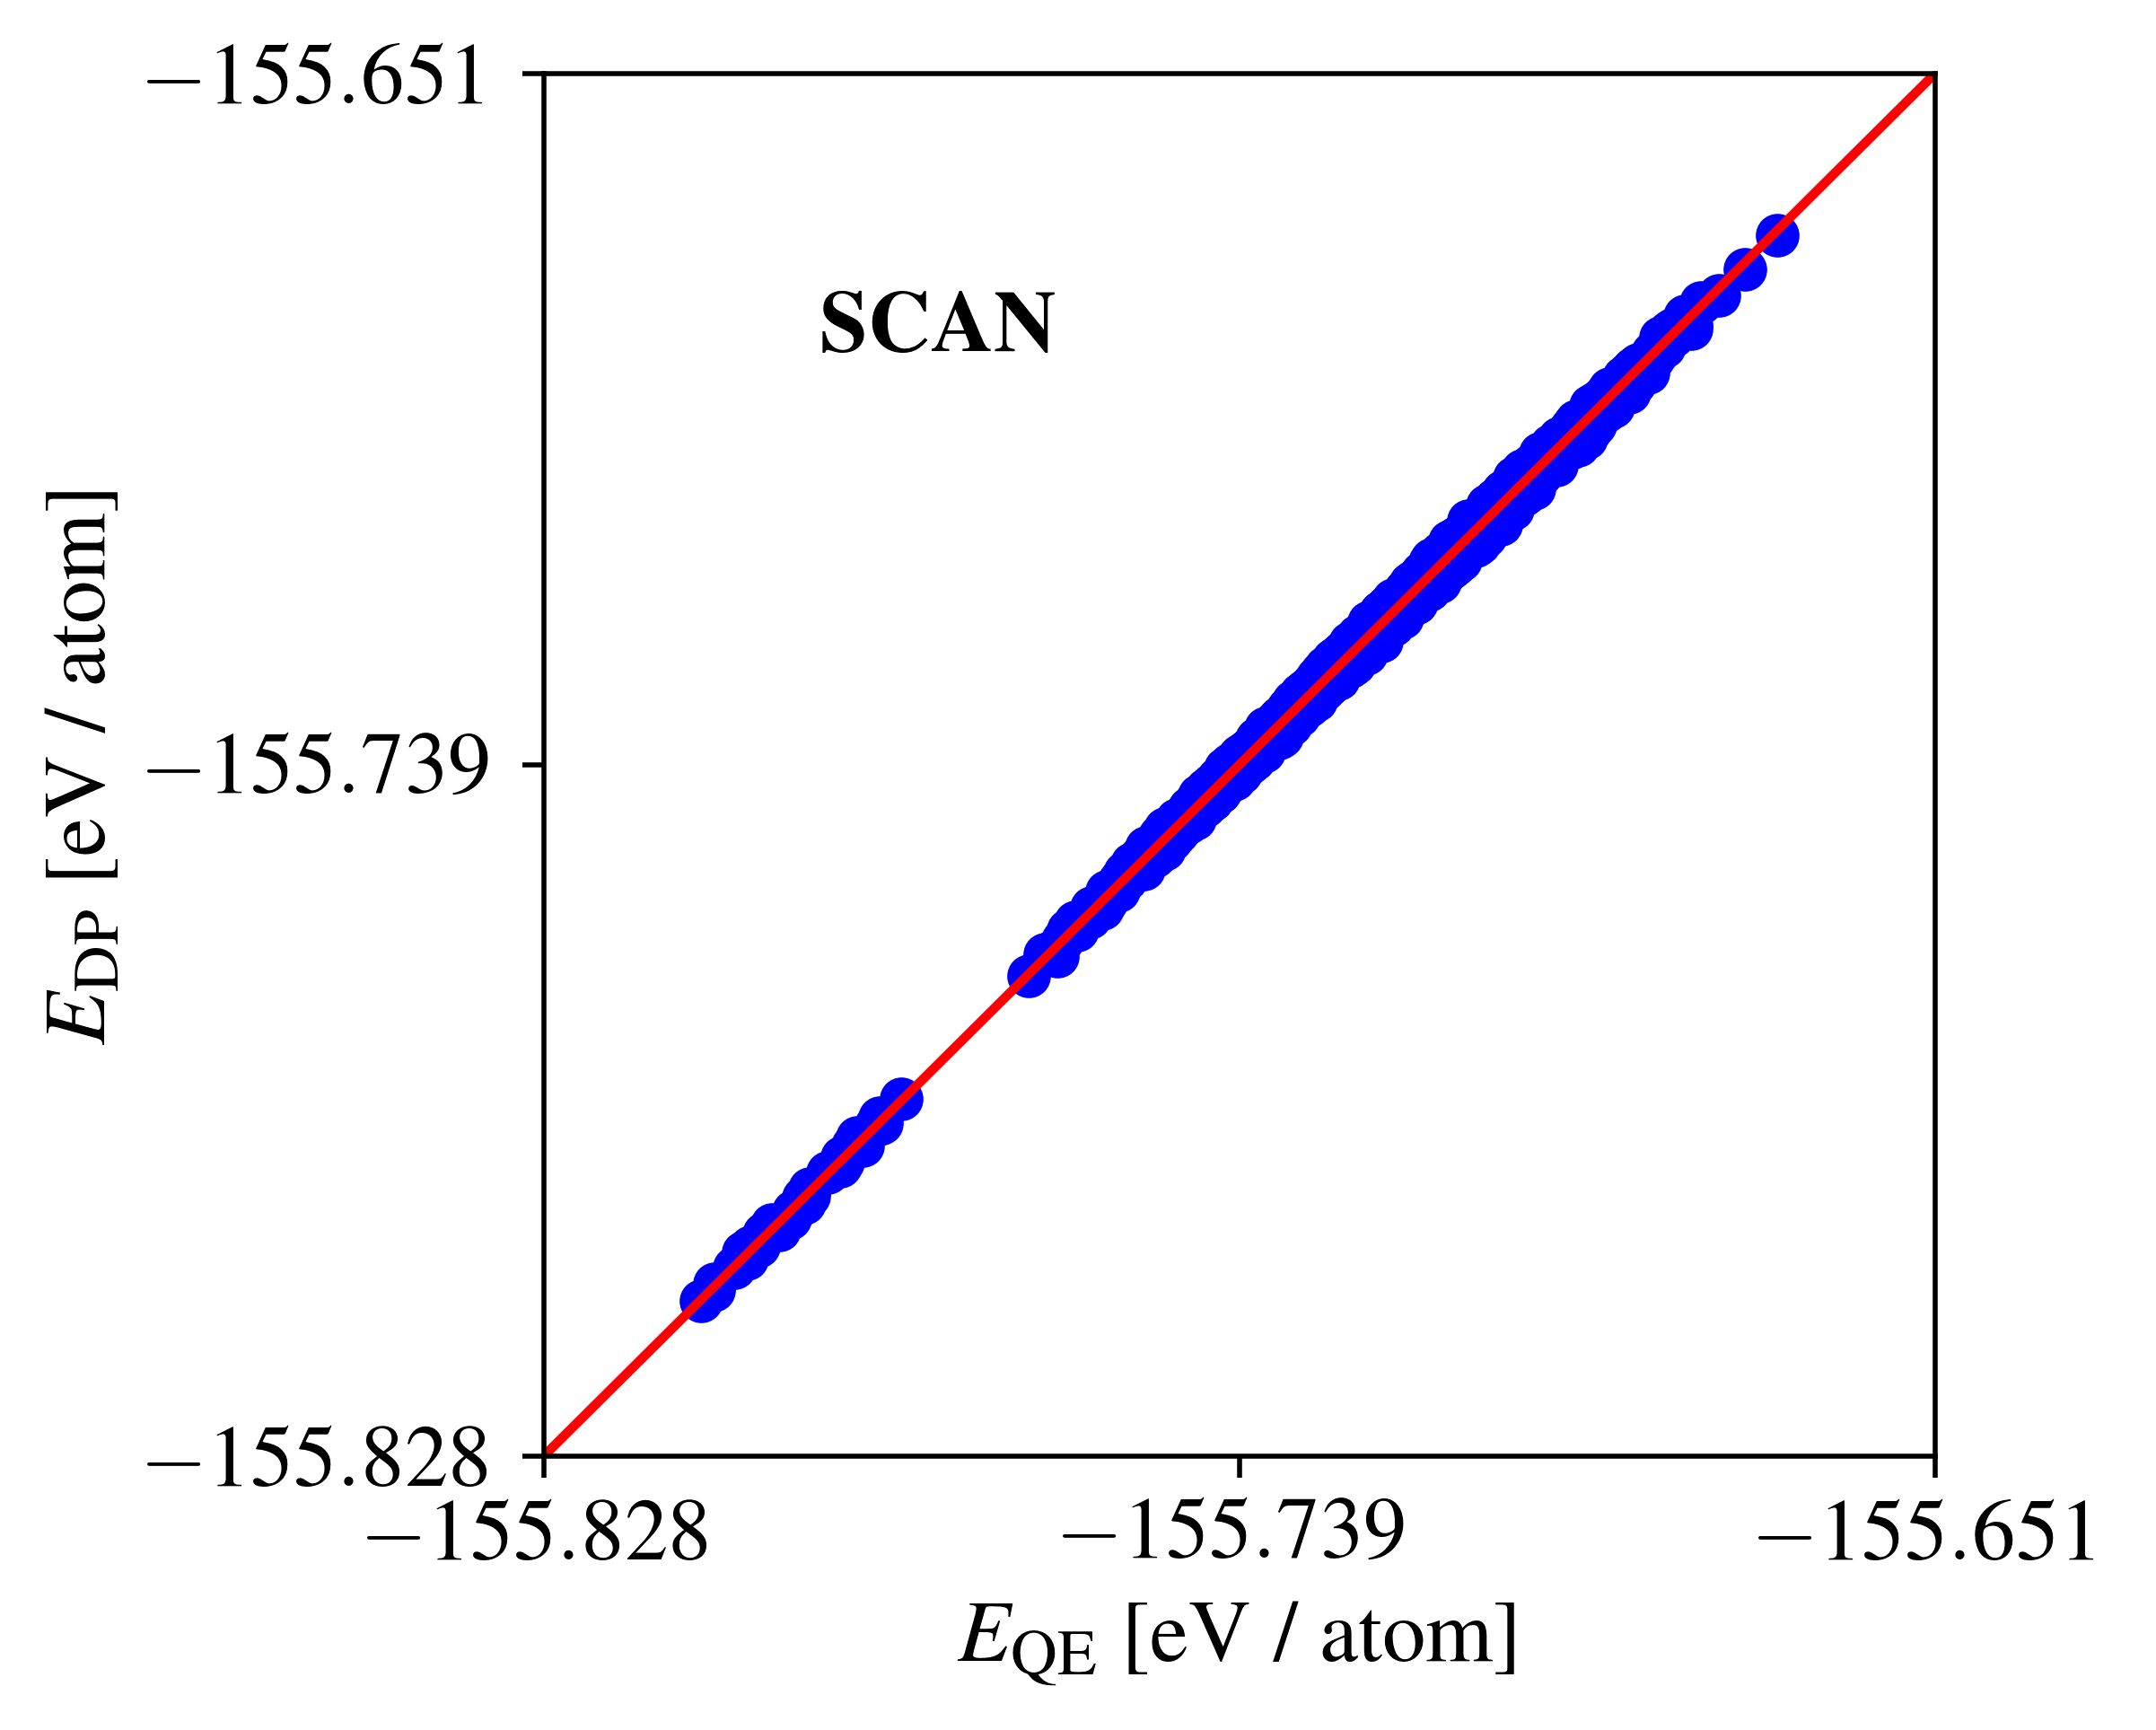}
\end{subfigure}
\hspace{0.1cm}
\begin{subfigure}[b]{0.45\linewidth}
\includegraphics[height=6cm]{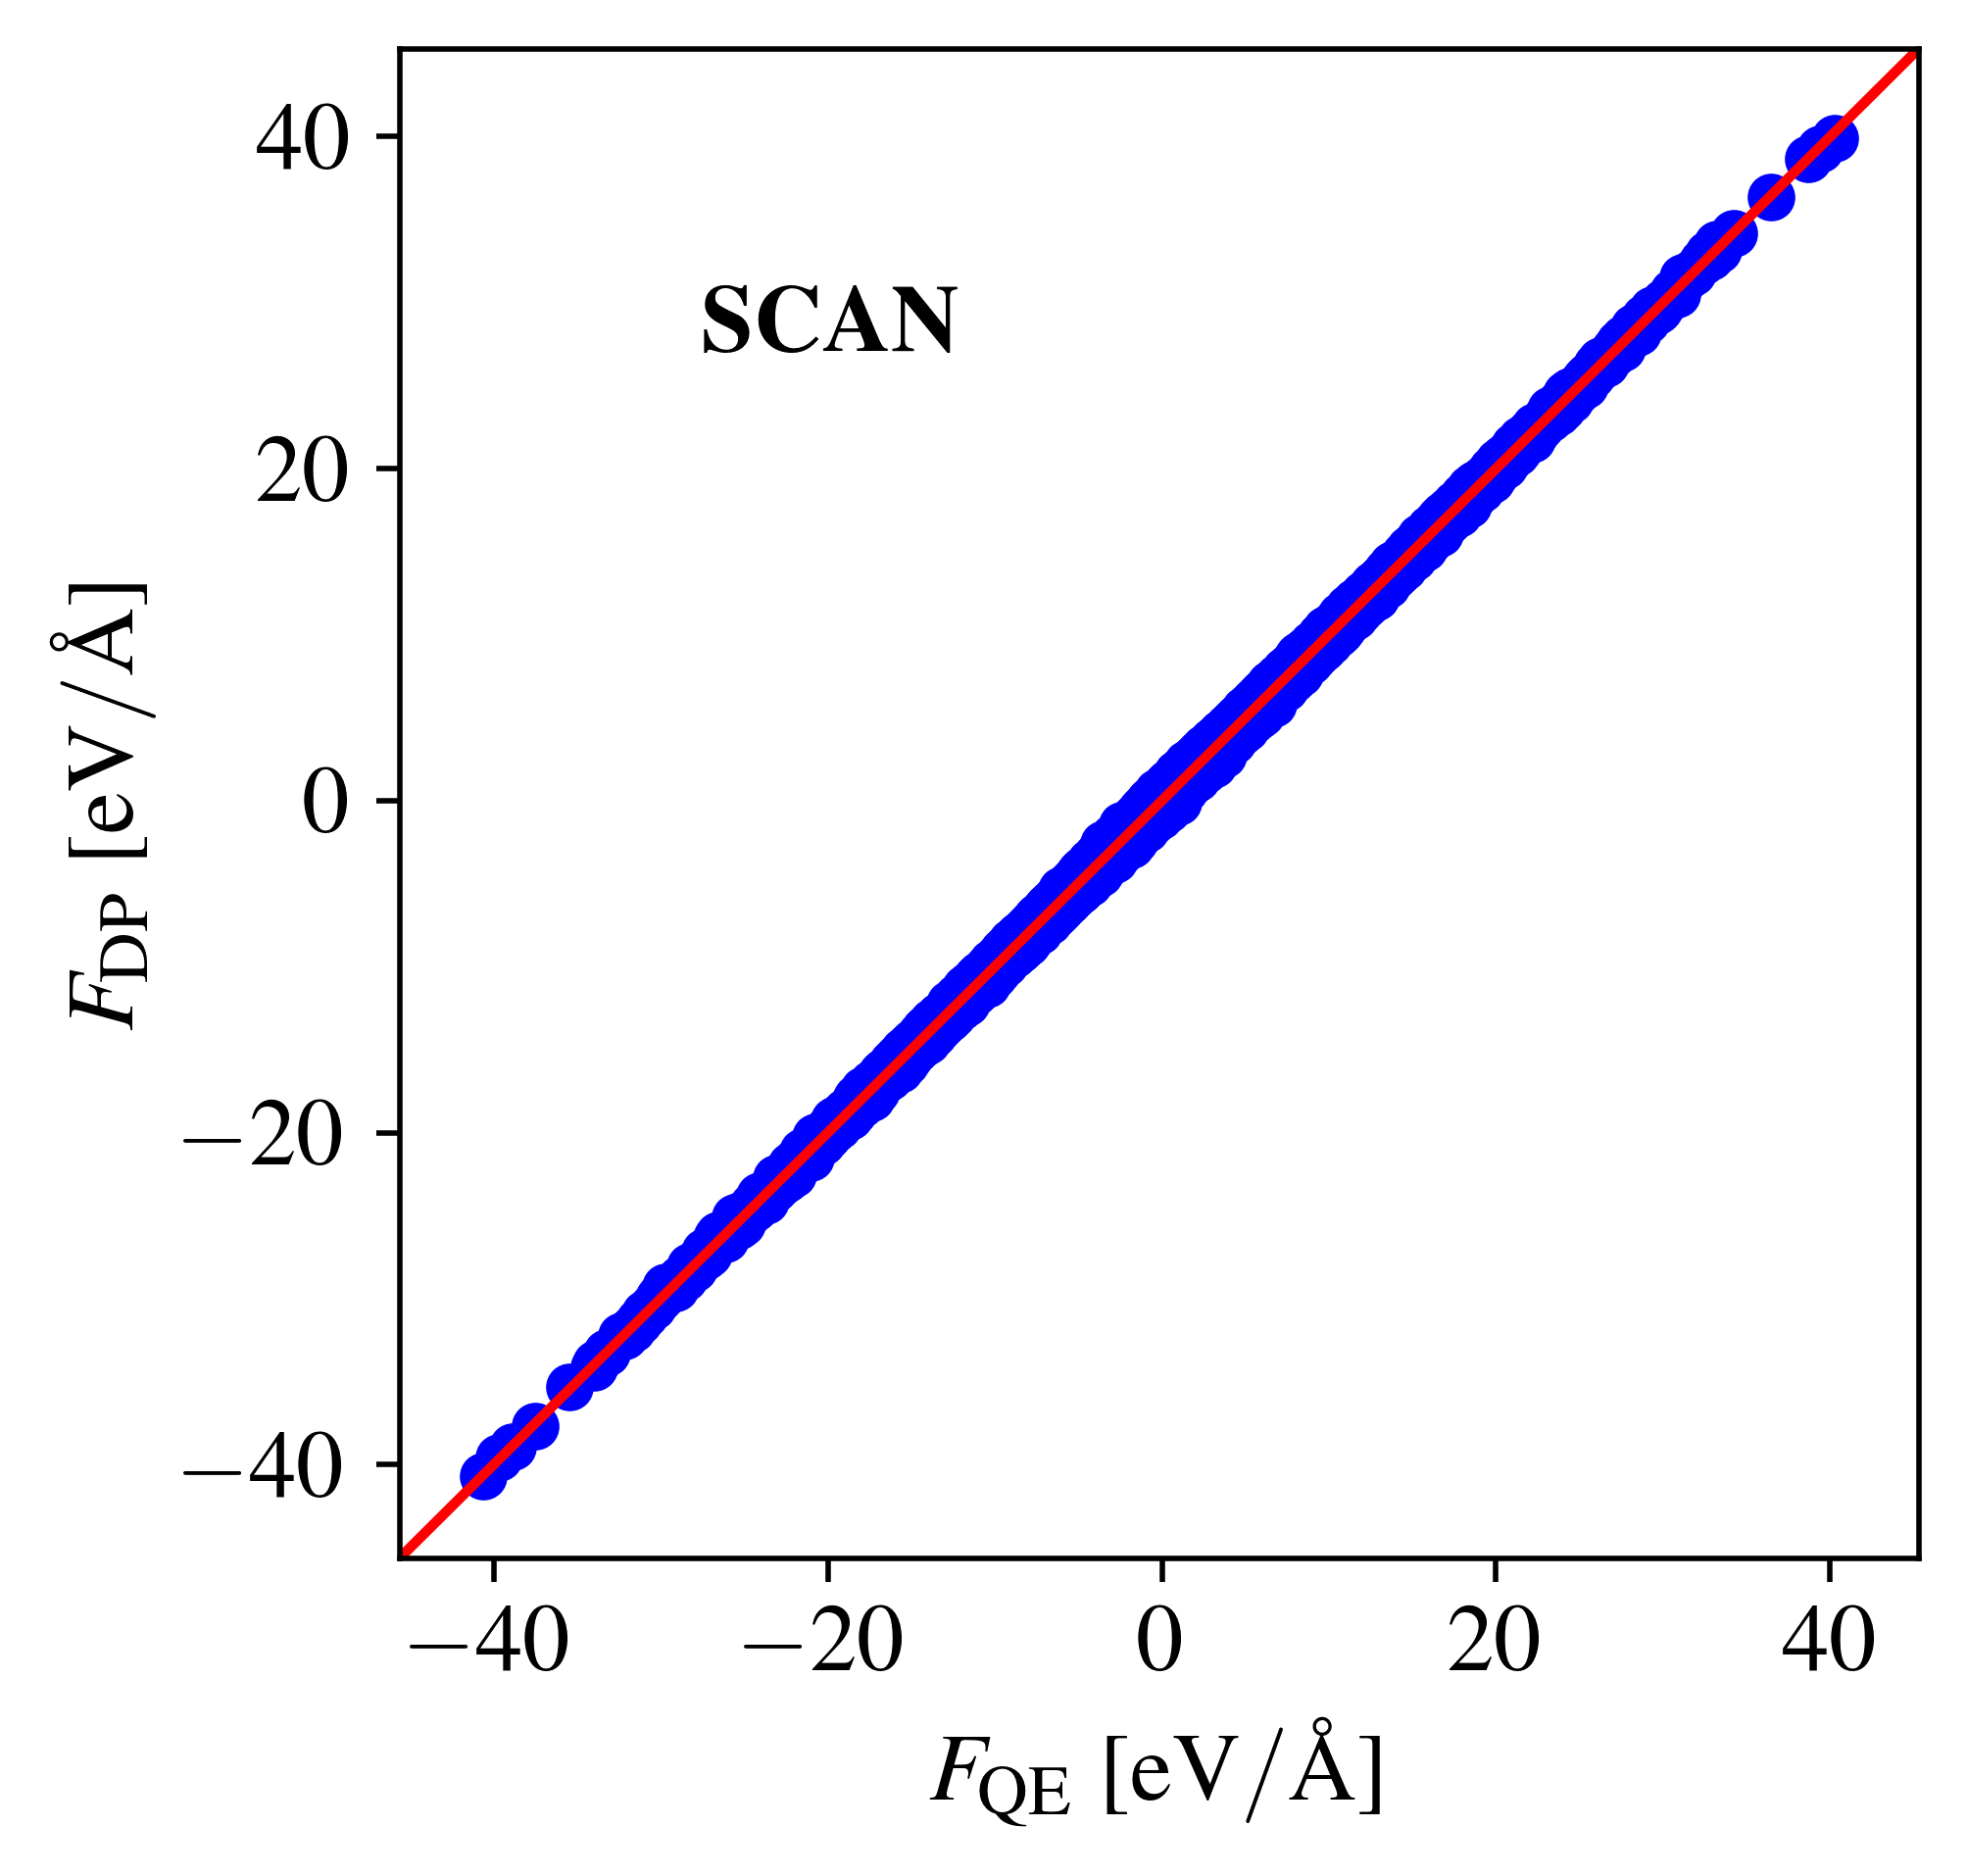}
\end{subfigure}

\vspace{0.1cm}

\begin{subfigure}[b]{0.45\linewidth}
\includegraphics[height=6cm]{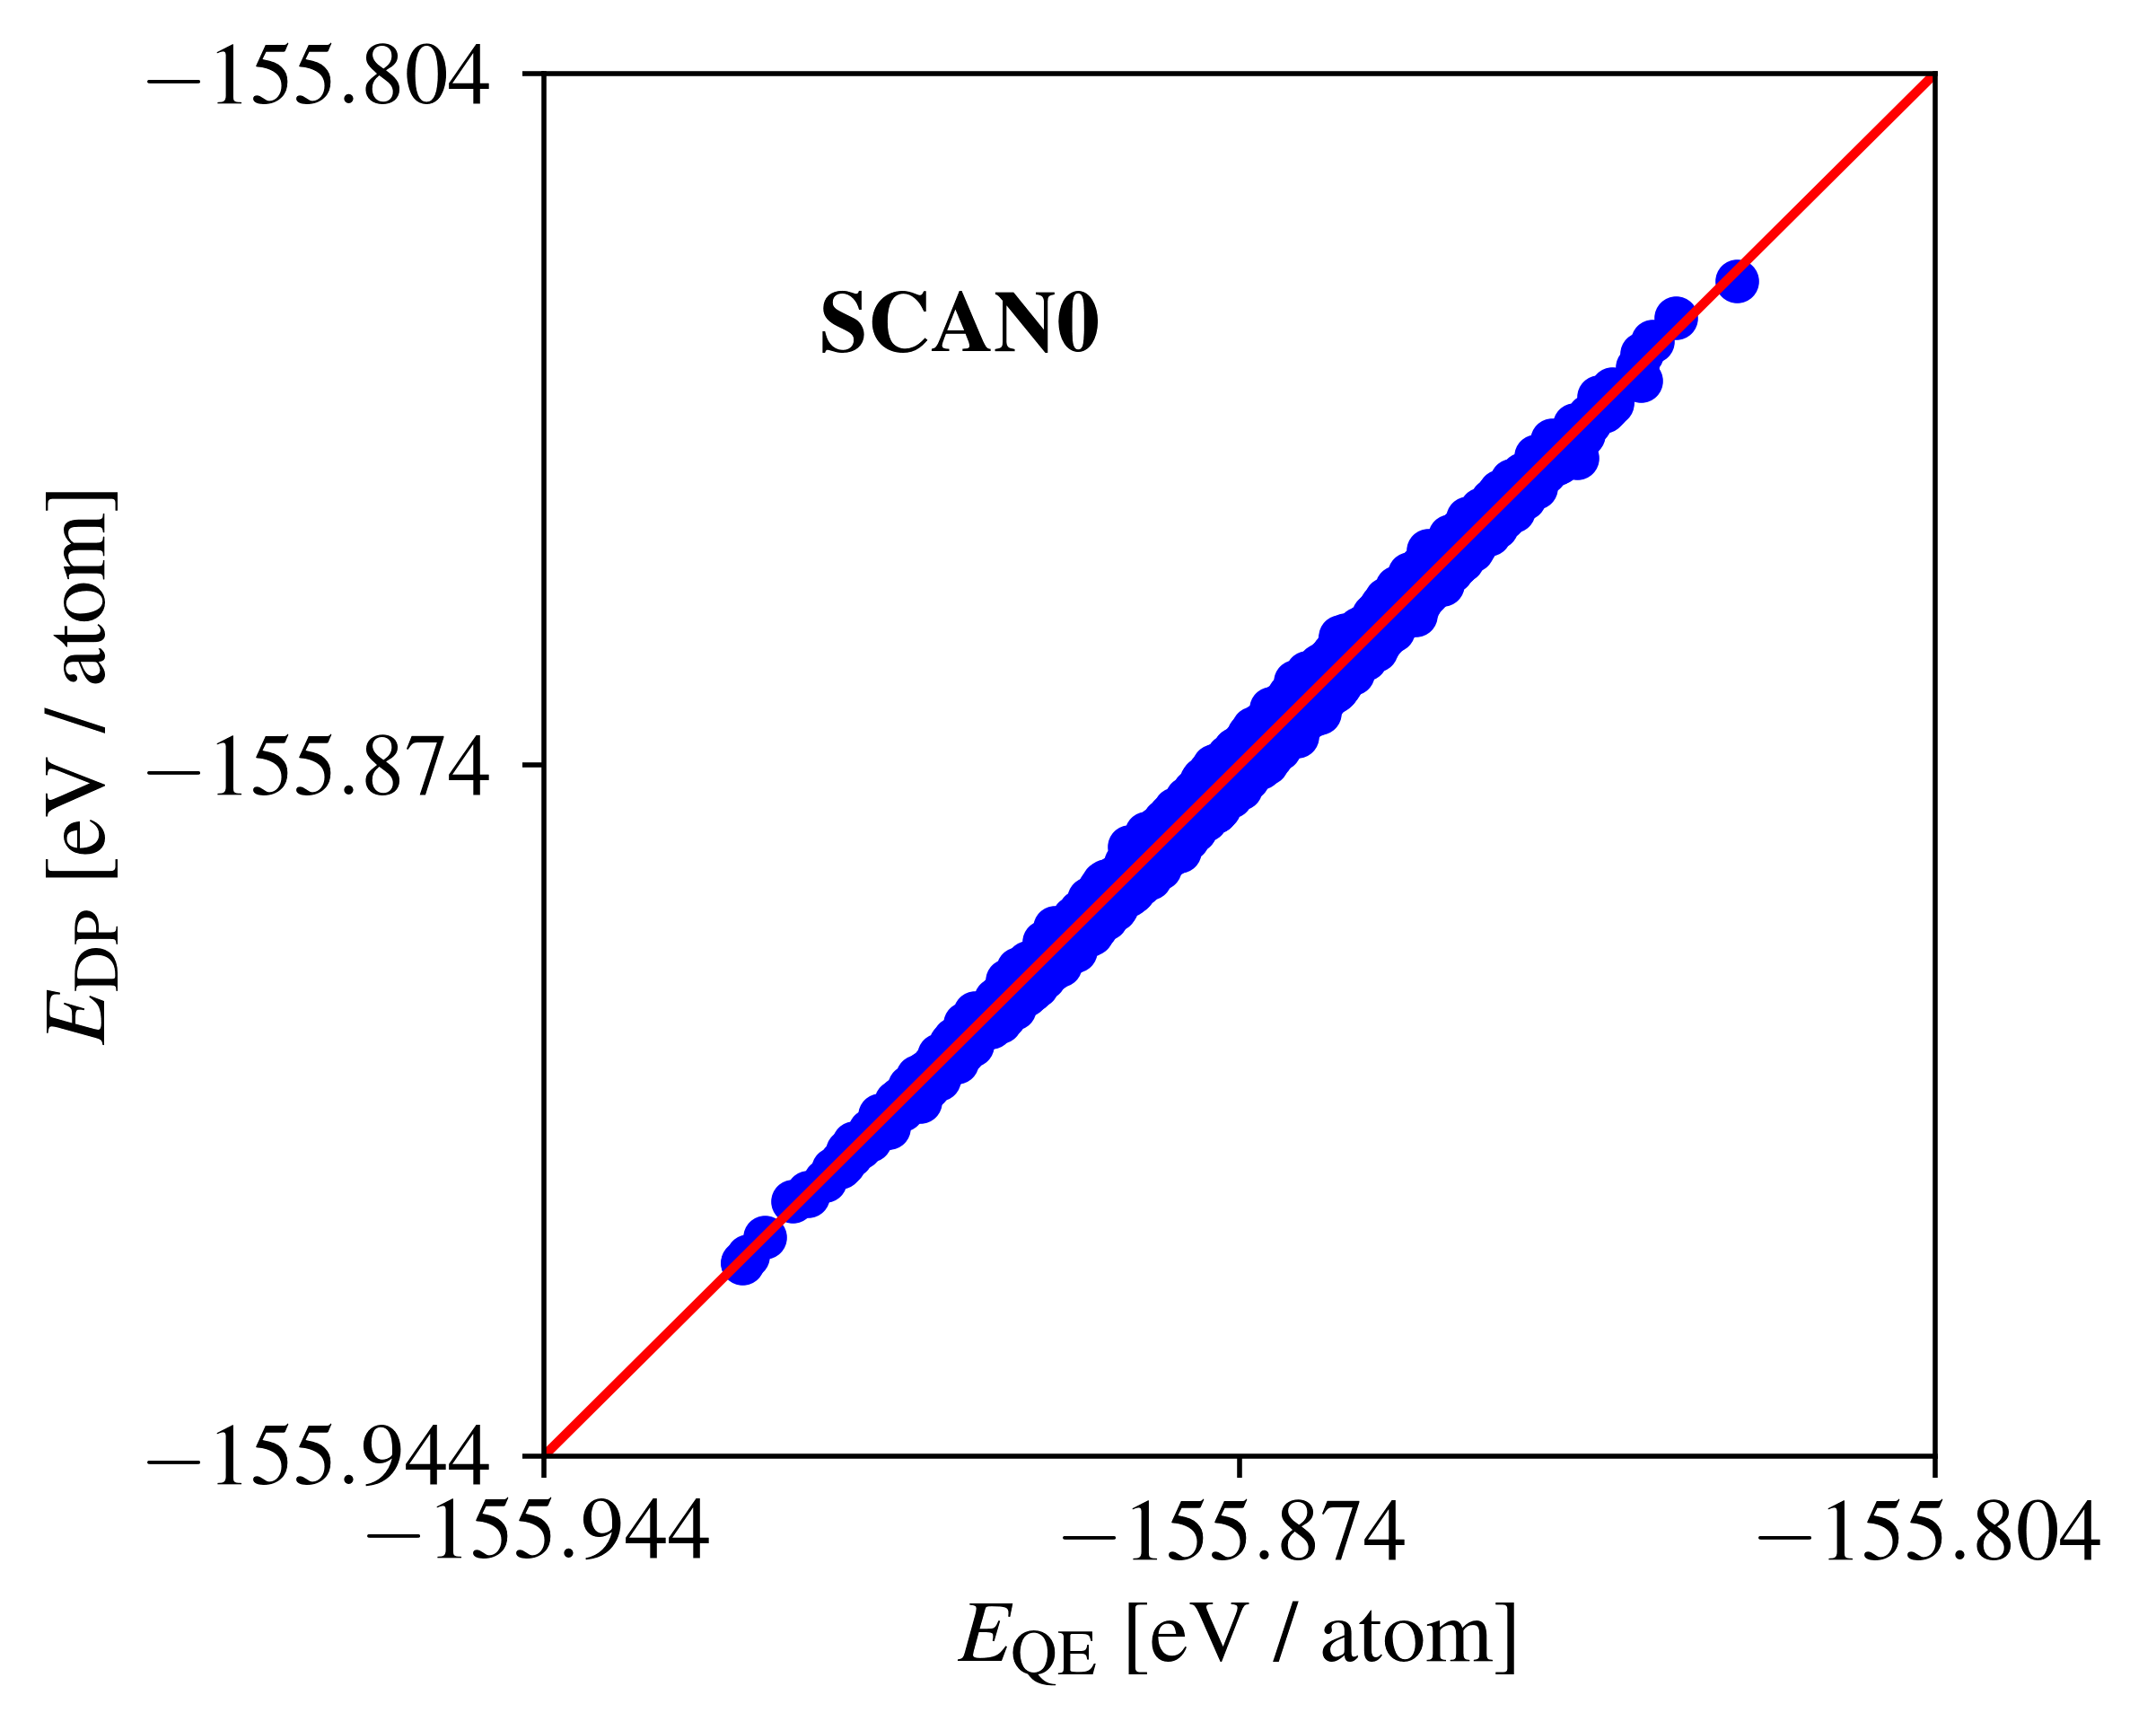}
\end{subfigure}
\hspace{0.1cm}
\begin{subfigure}[b]{0.45\linewidth}
\includegraphics[height=6cm]{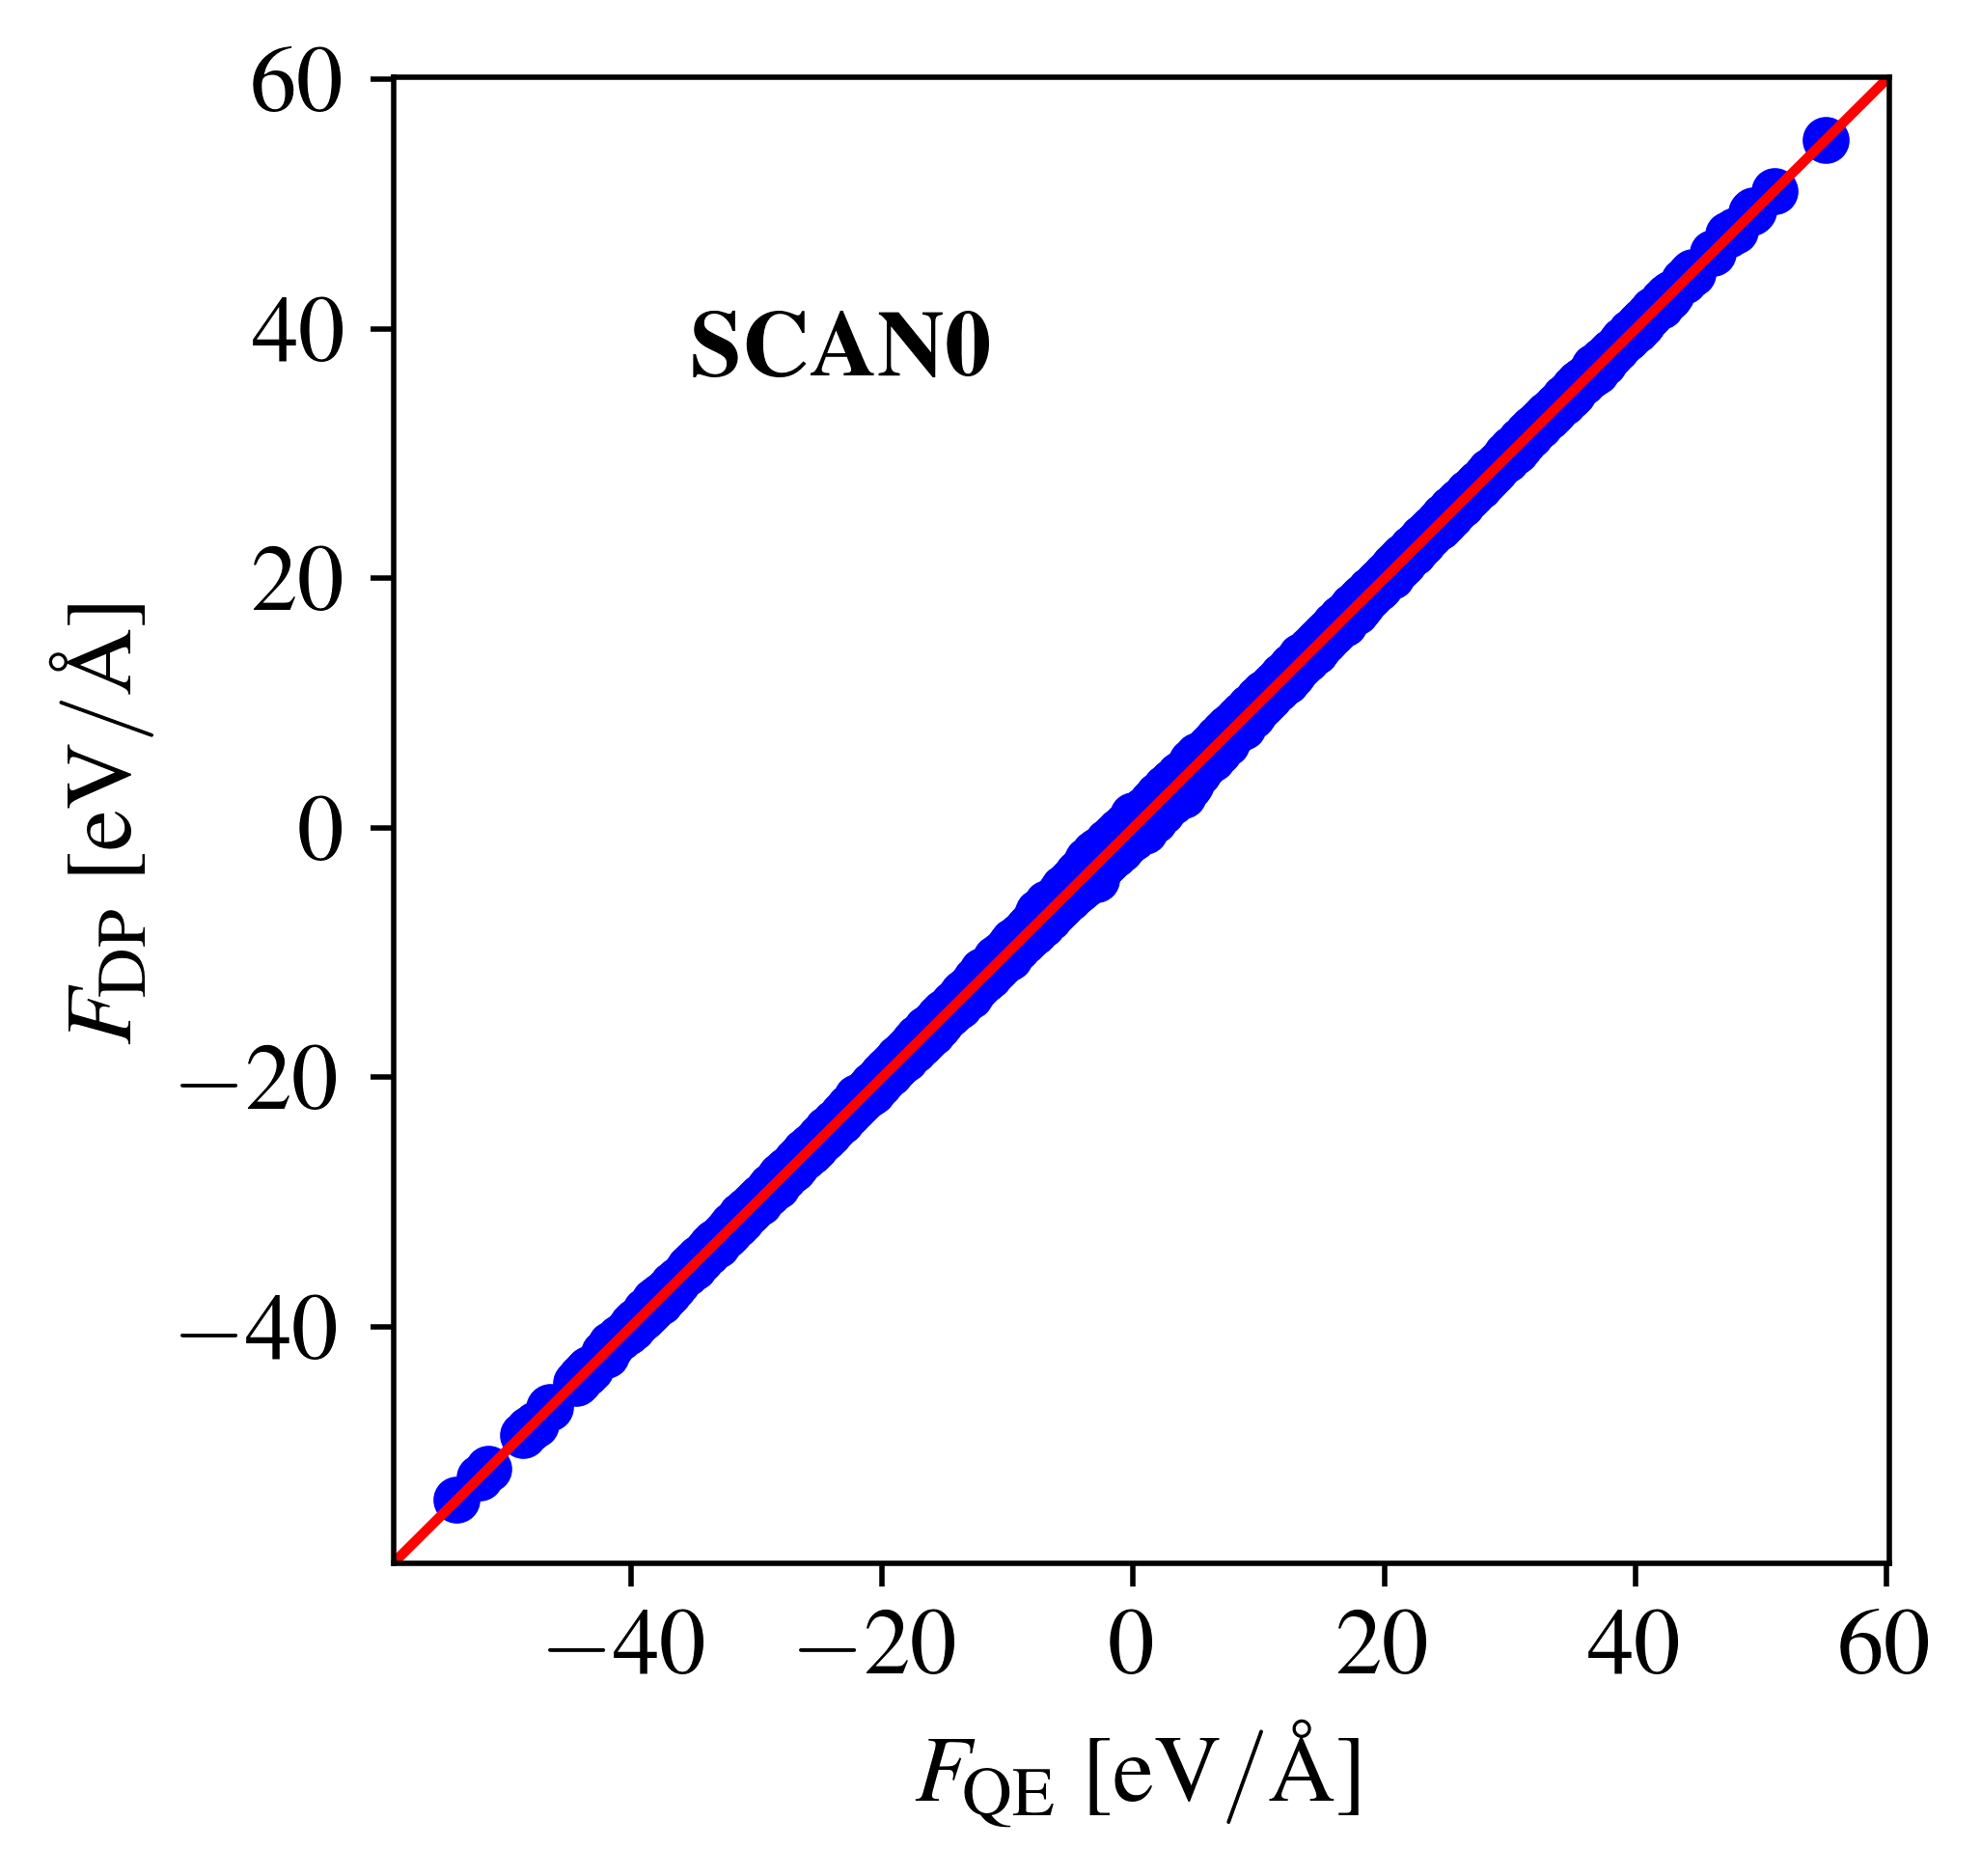}
\end{subfigure}
    \caption{DFT energies and forces compared with the values predicted by DP models.}
    \label{parity}
\end{figure}

% \section{Density of Ice and Water}\label{sm_density}
% \subsection{Calculations with DP Models}
% The density differences between water and ice Ih from classical MD (denoted as $\rho_{\mathrm{water}}^{\mathrm{cl}}-\rho_{\mathrm{ice\ Ih}}^{\mathrm{cl}}$) and PIMD (denoted as $\rho_{\mathrm{water}}^{\mathrm{qu}}-\rho_{\mathrm{ice\ Ih}}^{\mathrm{qu}}$) are reported in TABLE \ref{delta-dens}. We observe that at the melting temperature of ice Ih, the models based on SCAN, SCAN0, and MB-pol predict a density difference between water and ice close to the experimental value, while the models based on the revPBE-D3 and revPBE0-D3 functionals substantially underestimate the density difference.

% The temperature of maximum density of liquid water from classical MD (denoted as $T_{\mathrm{MD}}^{cl}$) and PIMD (denoted as $T_{\mathrm{MD}}^{cl}$) and their difference from the melting temperature of ice $\Delta T_{\mathrm{MD-m}}=T_{\mathrm{m}}-T_{\mathrm{MD}}$ are reported in TABLE \ref{tmd}. In experiment, the temperature of maximum density is +3.98 K higher than the melting temperature. The models based on MB-pol, SCAN, and SCAN0 qualitatively capture this effect, although they overestimate its value. The models based revPBE0-D3 and revPBE-D3 predict the temperature of maximum density to be lower than the melting temperature, which is in contrast with the experimental trend.

\pagebreak
\section{Classical thermodynamic integration}\label{sm_ti}
The chemical potentials calculated in Step 3, Hamiltonian Thermodynamic Integration, are listed in TABLE \ref{hti}.

% The third step is the HTI. At a given temperature $T_0$ and pressure $P_0$ (1 bar in this work), the Helmholtz free energies of ice and liquid water are calculated separately by performing the HTI from a reference state whose Helmholtz free energy can be calculated analytically. The reference states for liquid water and ice are the ideal gas of non-interacting water molecules and the Einstein crystal, respectively. The HTI precedure calculates the Helmholtz free energy difference between the target (ice or water) and the reference states by switching the coupling parameter between these two states. Accounting for the contributions of $P_0\langle V\rangle$, where $\langle V\rangle$ is the mean volume in the $NpT$ ensemble gives the Gibbs free energies at $T_0$ and $P_0$. The Gibbs free energies $G$ of water and ice calculated with the HTI are transformed to the chemical potential $\mu=\frac{G}{N}$, where $N$ is the number of water molecules. 

% In the HTI for ice or water, each path uses two intermediate states to avoid phase transition (see Section S II of the SM of Ref~\cite{zhang_phase_2021} for more discussions). The ``fix adapt/fep" method of LAMMPS is used to couple different interatomic interactions (for example, DP and the harmonic potential). For the the MD tasks in the HTI of ice we use the Langevin thermostat with a damping time of 0.1 ps to control the temperature. The MD tasks along the HTI path of liquid water use the Nos\'e-Hoover chain with a damping time of 0.1 ps. The chemical potentials calculated in the HTI step are listed in TABLE \ref{hti}.

\begin{table}[h!]
\caption{\label{hti}The Chemical Potential $\mu$ of Water and Ice at 1 bar Calculated with HTI\footnote{The value in parentheses is the statistical uncertainty in the last digit.}}
\begin{tabular}{ccccc}
\hline
Model & Phase & $T_{\mathrm{init}}$ [K] & $P$ [bar] & $\mu(P, T_{\mathrm{init}})$ [eV / H$_2$O]\\ \hline
DP@revPBE-D3 &  Ice Ih &  150  &  1 & -468.0095 (2)  \\
DP@revPBE-D3 &  Ice Ih &  300  &  1 & -467.9641 (4)  \\
DP@revPBE-D3 &  Water  &  300  &  1 & -467.9641 (1)  \\
DP@revPBE-D3 &  Water  &  350  &  1 & -467.9817 (1)  \\
\hline
DP@revPBE0-D3 &  Ice Ih &  150  &  1 & -469.3987 (2) \\
DP@revPBE0-D3 &  Ice Ih &  300  &  1 & -469.3517 (4)  \\
DP@revPBE0-D3 &  Water  &  300  &  1 & -469.3526 (2)  \\
DP@revPBE0-D3 &  Water  &  350  &  1 & -469.3701 (2)  \\
\hline
DP@SCAN &  Ice Ih &  150  &  1 & -467.3948 (2)  \\
DP@SCAN &  Ice Ih &  300  &  1 & -467.3439 (4)  \\
DP@SCAN &  Water  &  300  &  1 & -467.3409 (2)  \\
DP@SCAN &  Water  &  350  &  1 & -467.3535 (2)  \\
\hline
DP@SCAN0 &  Ice Ih &  150  &  1 & -467.9174 (2)  \\
DP@SCAN0 &  Ice Ih &  300  &  1 & -467.8666 (4)  \\
DP@SCAN0 &  Water  &  300  &  1 & -467.8636 (2)  \\
DP@SCAN0 &  Water  &  350  &  1 & -467.8764 (2)  \\
\hline
\end{tabular}%
\end{table}

% The fourth step is the TI along a temperature path starting from the Gibbs free energy at $T_0$. The output of this step is the chemical potentials of ice and water at different temperatures. We plot the temperature-dependent chemical potential curves $\mu(T)$ of ice and water for different models in FIG. \ref{mu_t}. To ensure the correctness of our TI, we do the \textit{consistency check}. We perform the HTI at two different temperatures for each calculation and start at two $T_0$ values in each TI path along the temperature. The two $\mu(T)$ curves from independent TI calculations with different $T_0$ match with each other, demonstrating that our TI calculation is correct.

% The temperature-dependent chemical potential differences between water and ice, $\Delta \mu_{\mathrm{liq} \rightarrow \mathrm{ice}}^{\mathrm{classical}}(T)$, are reported in FIG. \ref{chemical_potential} as blue lines. The classical melting temperature is given by the $T$ value for which $\Delta \mu_{\mathrm{liq} \rightarrow \mathrm{ice}}^{\mathrm{classical}}(T)=0$.

\pagebreak
\section{Mass Thermodynamic Integration at Different Temperatures}\label{sm_mti_temps}
We report the $\Delta g_{\mathrm{ice} - \mathrm{liq}}(y)$ curves at different temperatures in FIG. \ref{integrand}. % By integrating $g(y)$ on $y\in(0, 1)$ numerically with the trapezoidal rule, we calculate $\Delta\Delta\mu_{\mathrm{liq} \rightarrow \mathrm{ice}}(T)$, which is reported in FIG. \ref{sm_ddmu}. The difference between the chemical potentials of quantum ice and water is calculated with $\Delta \mu_{\mathrm{liq} \rightarrow \mathrm{ice}}^{\mathrm{quantum}}(T)=\Delta \mu_{\mathrm{liq} \rightarrow \mathrm{ice}}^{\mathrm{classical}}(T)+\Delta\Delta\mu_{\mathrm{liq} \rightarrow \mathrm{ice}}(T)$ and reported in FIG. \ref{chemical_potential}. The classical and quantum melting points are the temperatures where $\Delta \mu_{\mathrm{liq} \rightarrow \mathrm{ice}}^{\mathrm{classical}}(T)=0$ and $\Delta \mu_{\mathrm{liq} \rightarrow \mathrm{ice}}^{\mathrm{quantum}}(T)=0$, respectively.
\begin{figure}[h!]
     \centering
     \includegraphics[width=0.8\textwidth]{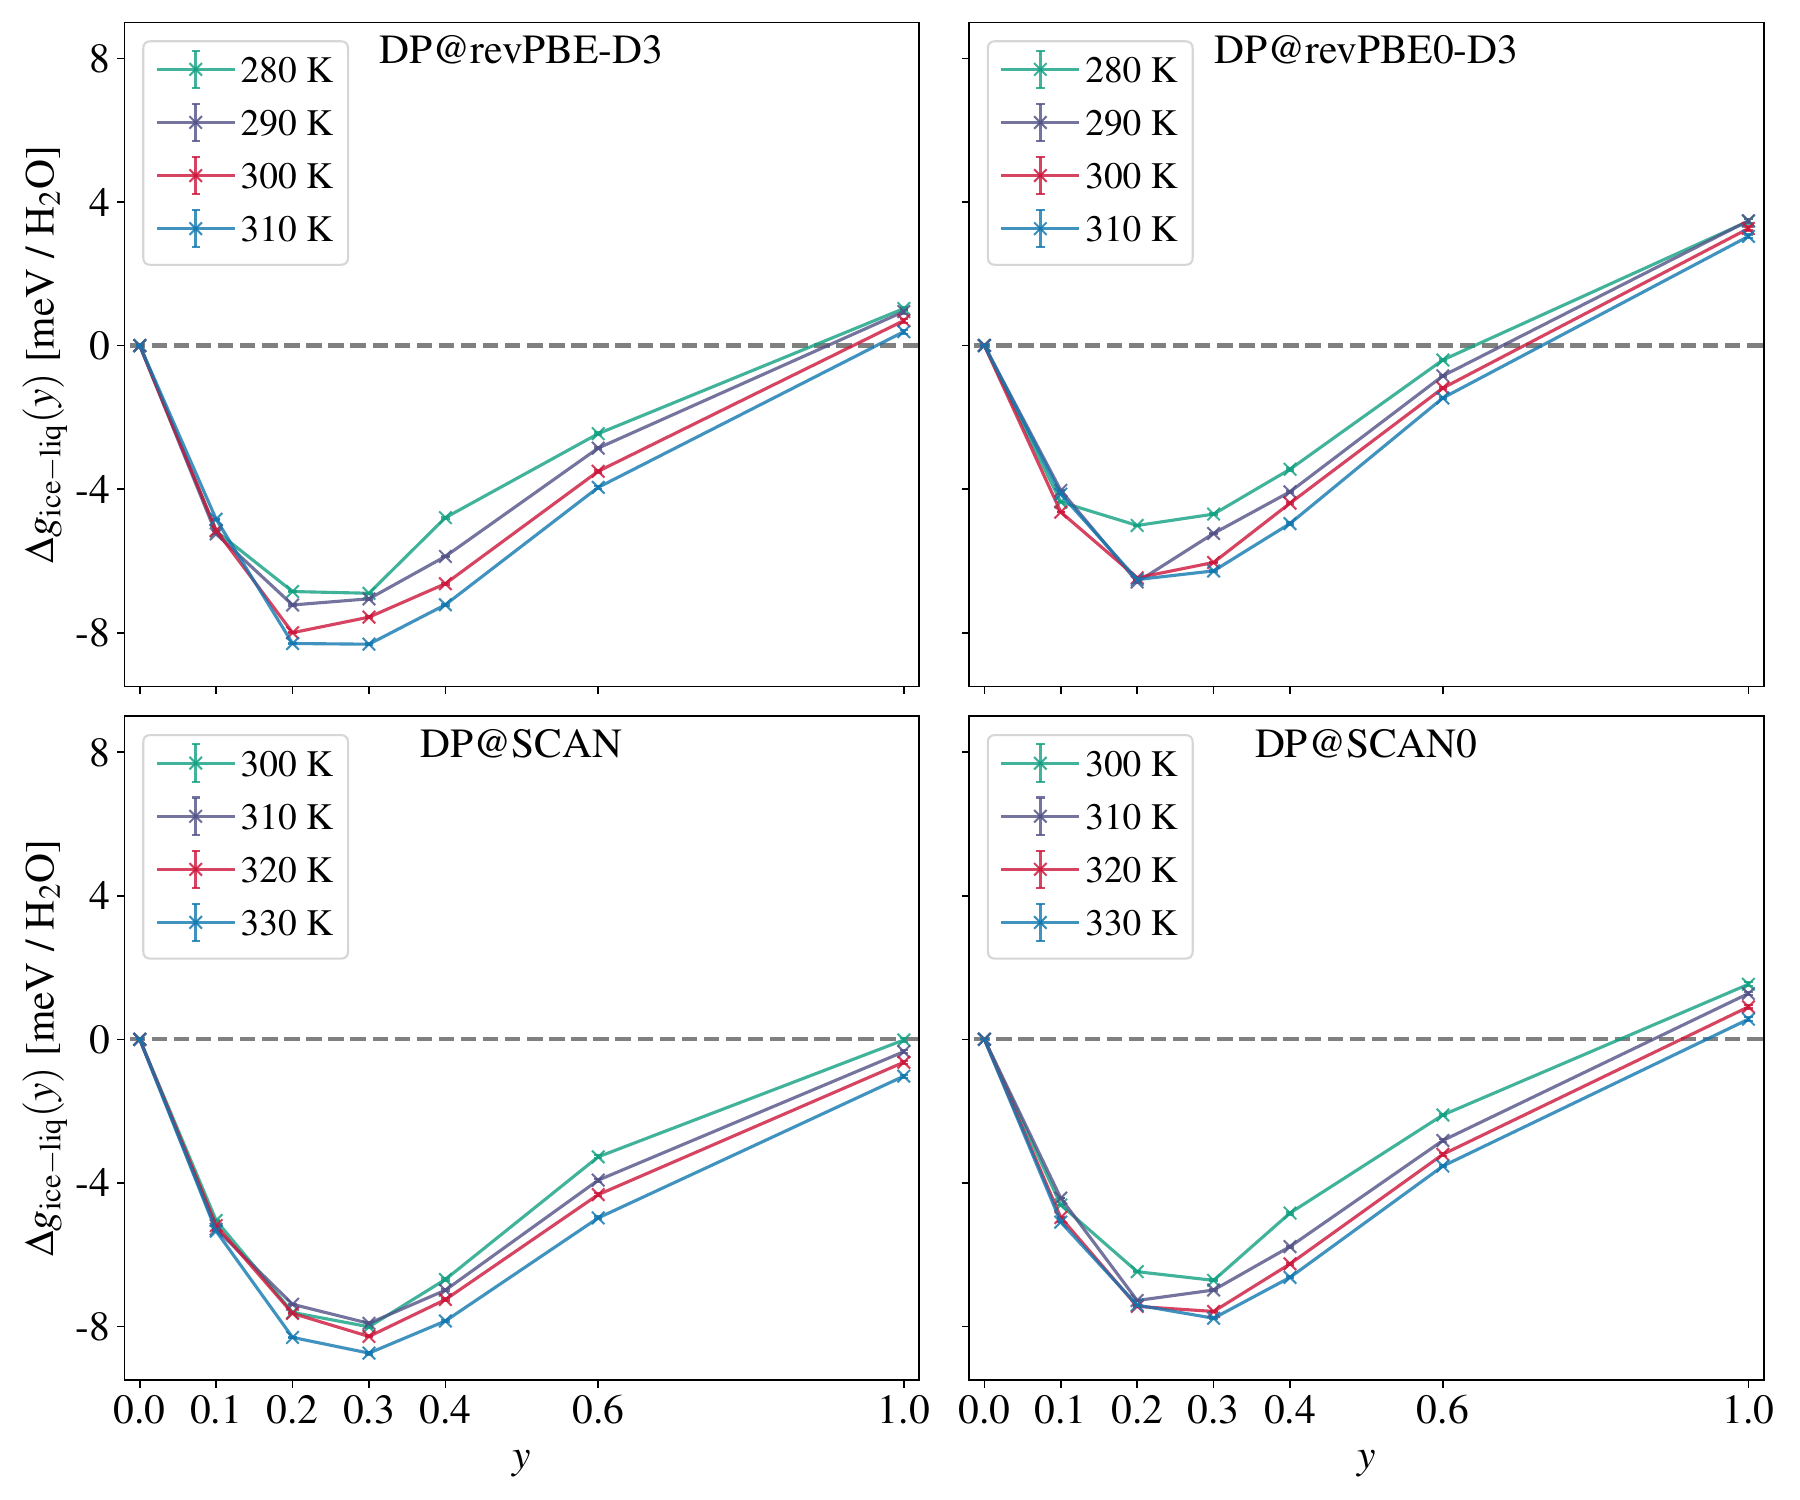}
     % \begin{subfigure}[b]{0.48\textwidth}
     %     \centering
     %     \includegraphics[width=\textwidth]{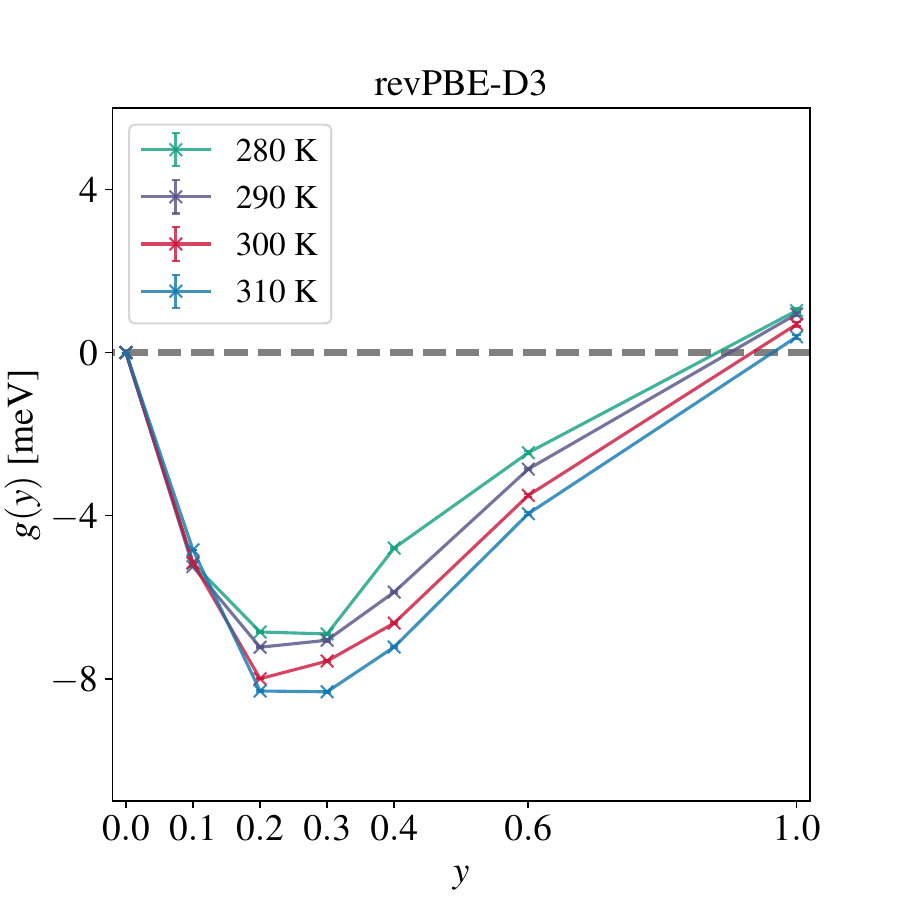}
     % \end{subfigure}
     % \begin{subfigure}[b]{0.48\textwidth}
     %     \centering
     %     \includegraphics[width=\textwidth]{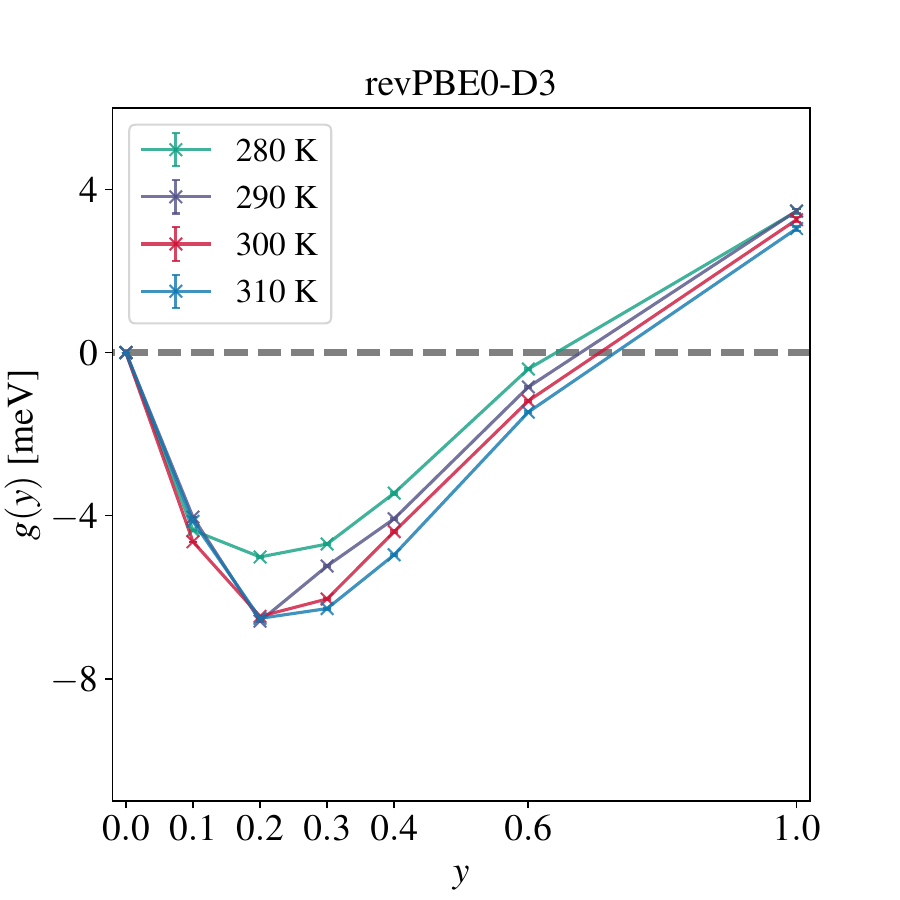}
     % \end{subfigure}
     % \begin{subfigure}[b]{0.48\textwidth}
     %     \centering
     %     \includegraphics[width=\textwidth]{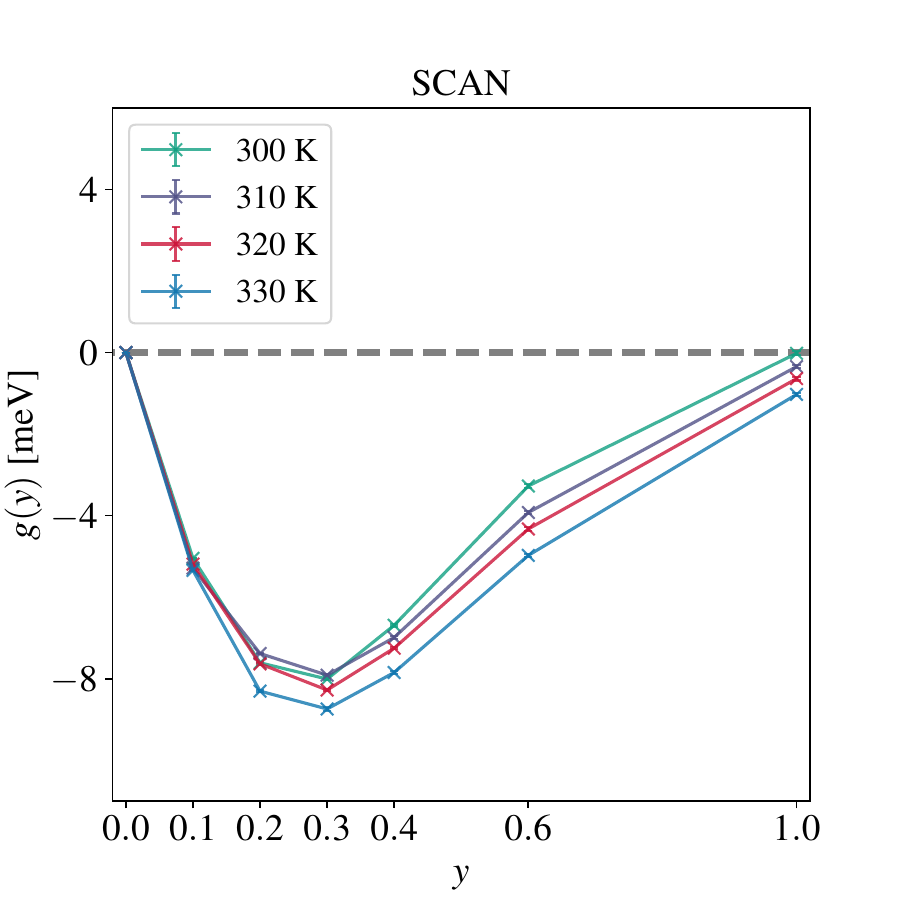}
     % \end{subfigure}
     % \begin{subfigure}[b]{0.48\textwidth}
     %     \centering
     %     \includegraphics[width=\textwidth]{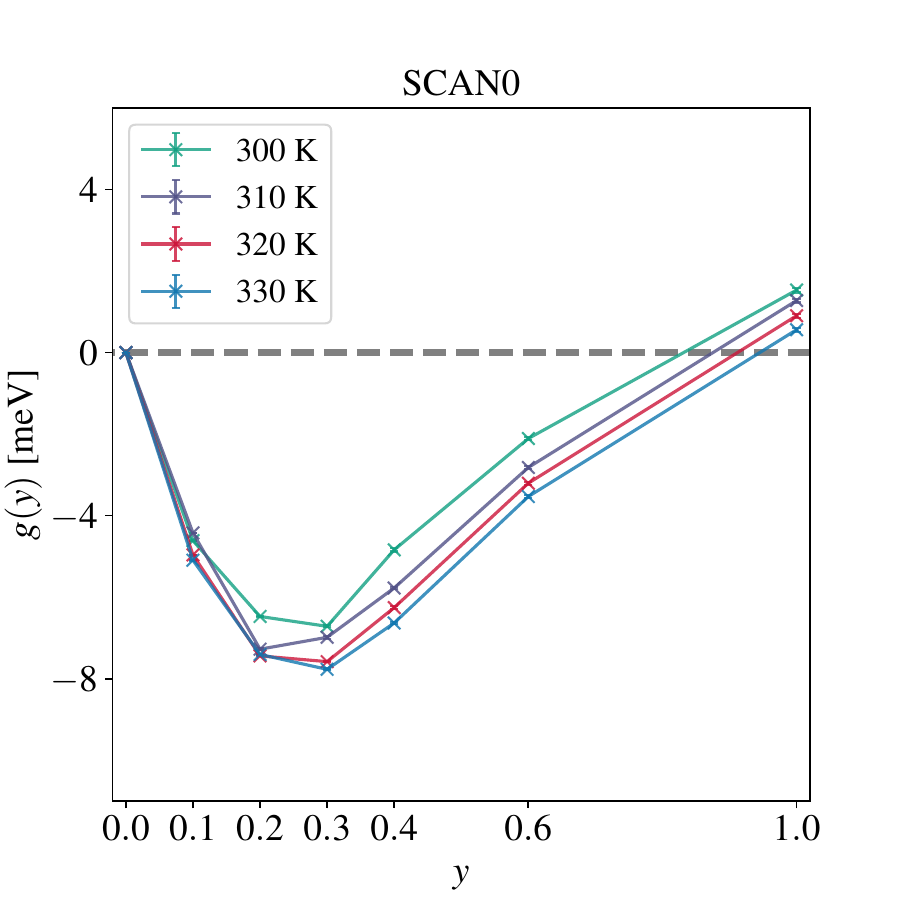}
     % \end{subfigure}
    \caption{$\Delta g_{\mathrm{ice} - \mathrm{liq}}(y)$ curves for each functional at different temperatures around the melting point. }
    \label{integrand}
\end{figure}

\pagebreak
\section{Mass Thermodynamic Integration with Reduced Number of Beads}\label{mti_reduced_beads}
We validate the $T_{\mathrm{m}}$ for DP@SCAN obtained with the direct coexistence method by performing the mass thermodynamic integration calculation with reduced number of beads, i.e., 8, 16, 32, 32, 32, 32 for $y=0.1$, 0.2, 0.3, 0.4, 0.6, 1.0, respectively.
\begin{figure*}[ht!]
     \centering
     \begin{subfigure}[b]{0.46\textwidth}
         \centering
         \includegraphics[width=\textwidth]{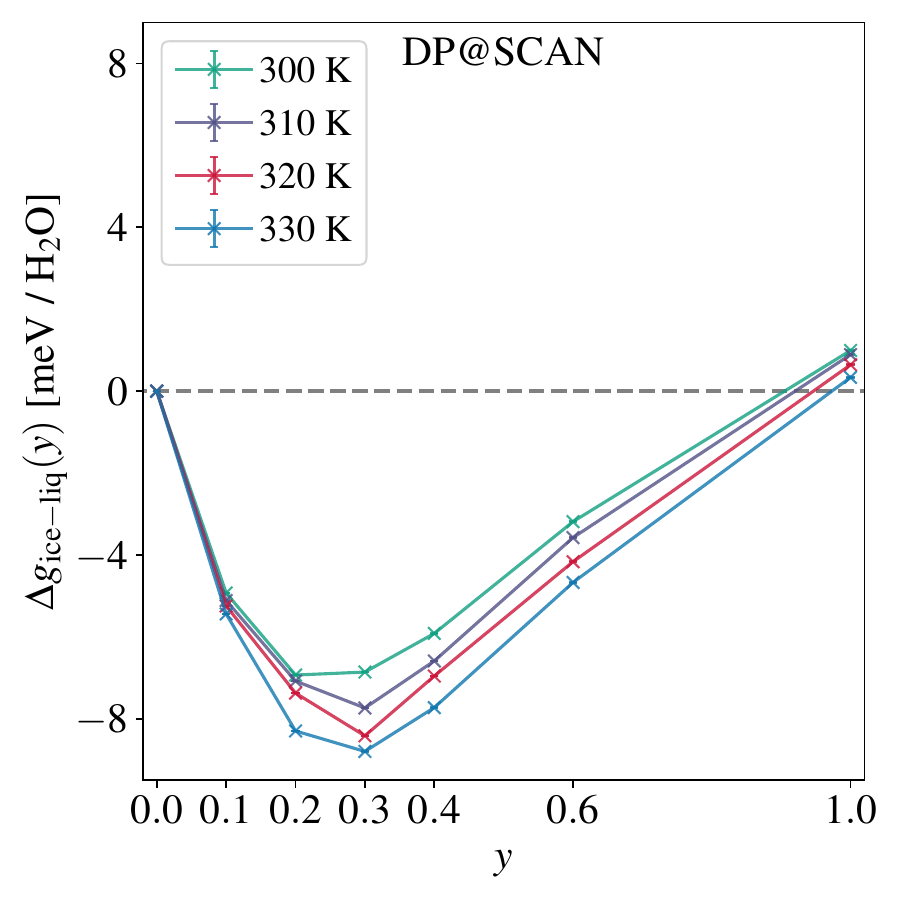}
         % \captionsetup{justification=raggedright,singlelinecheck=off}
         \caption{$\Delta g_{\mathrm{ice} - \mathrm{liq}}(y)$ curves for SCAN with reduced number of beads at different temperatures around the melting point. }
         % \raisebox{15pt}{\makebox[\linewidth][l]{(a)}} 
         \label{int5}
     \end{subfigure}
     \hspace{0.1cm}
     \begin{subfigure}[b]{0.45\textwidth}
         \centering
         \includegraphics[width=\textwidth]{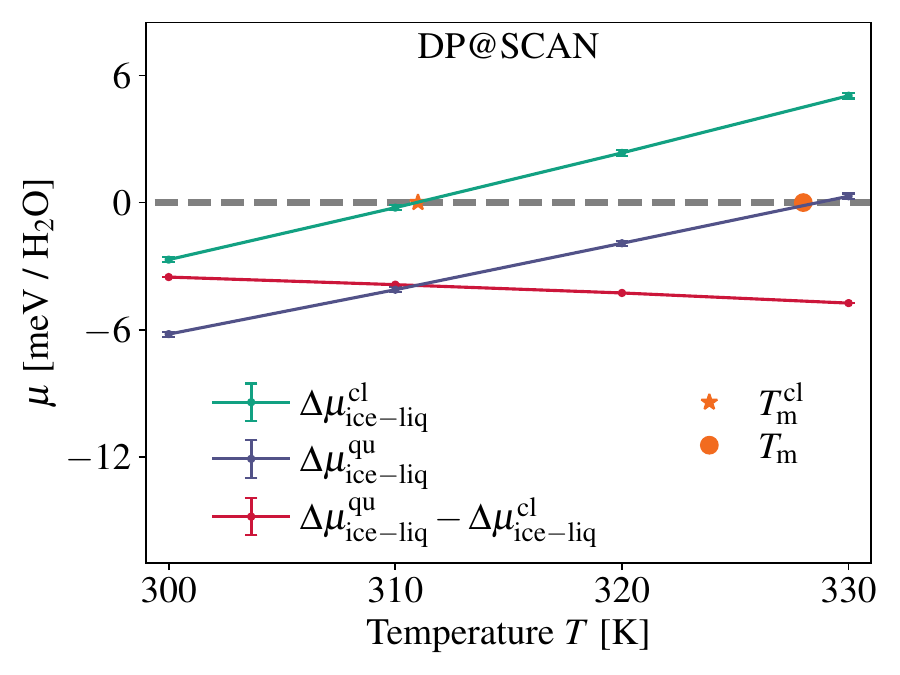}
         % \caption{The initial and final states of the direct coexistence simulation are demonstrated. The coexisting ice and water system tend to thaw at high temperatures, and ice grows at low temperatures.}
         % \captionsetup{justification=raggedright,singlelinecheck=off}
         \caption{The chemical potential differences obtained with reduced number of beads.}
         % \raisebox{15pt}{\makebox[\linewidth][l]{(b)}} 
         \label{mu5}
     \end{subfigure}
\caption{The mass thermodynamic integration result for DP@SCAN with reduced number of beads. The chemical potential differences yield $T_{\mathrm{m}}=328\pm 1$ K, which is slightly lower than $T_{\mathrm{m}}=330\pm 1$ K obtained with fully converged numbers of beads, and agrees with $T_{\mathrm{m}}=324\pm 3$ K obtained in the direct coexistence simulations within error bar.}
\label{32beads}
\end{figure*}

\end{document}
